# Supplementary material for: Viewpoint Textual Inversion: Discovering Scene Representations and 3D View Control in 2D Diffusion Models
Source: arXiv:2309.07986 source file (2024-07-26)
Supplement: Supplementary file 1 [file figs-viewneti-latex-supp-resolutiongood.pdf]

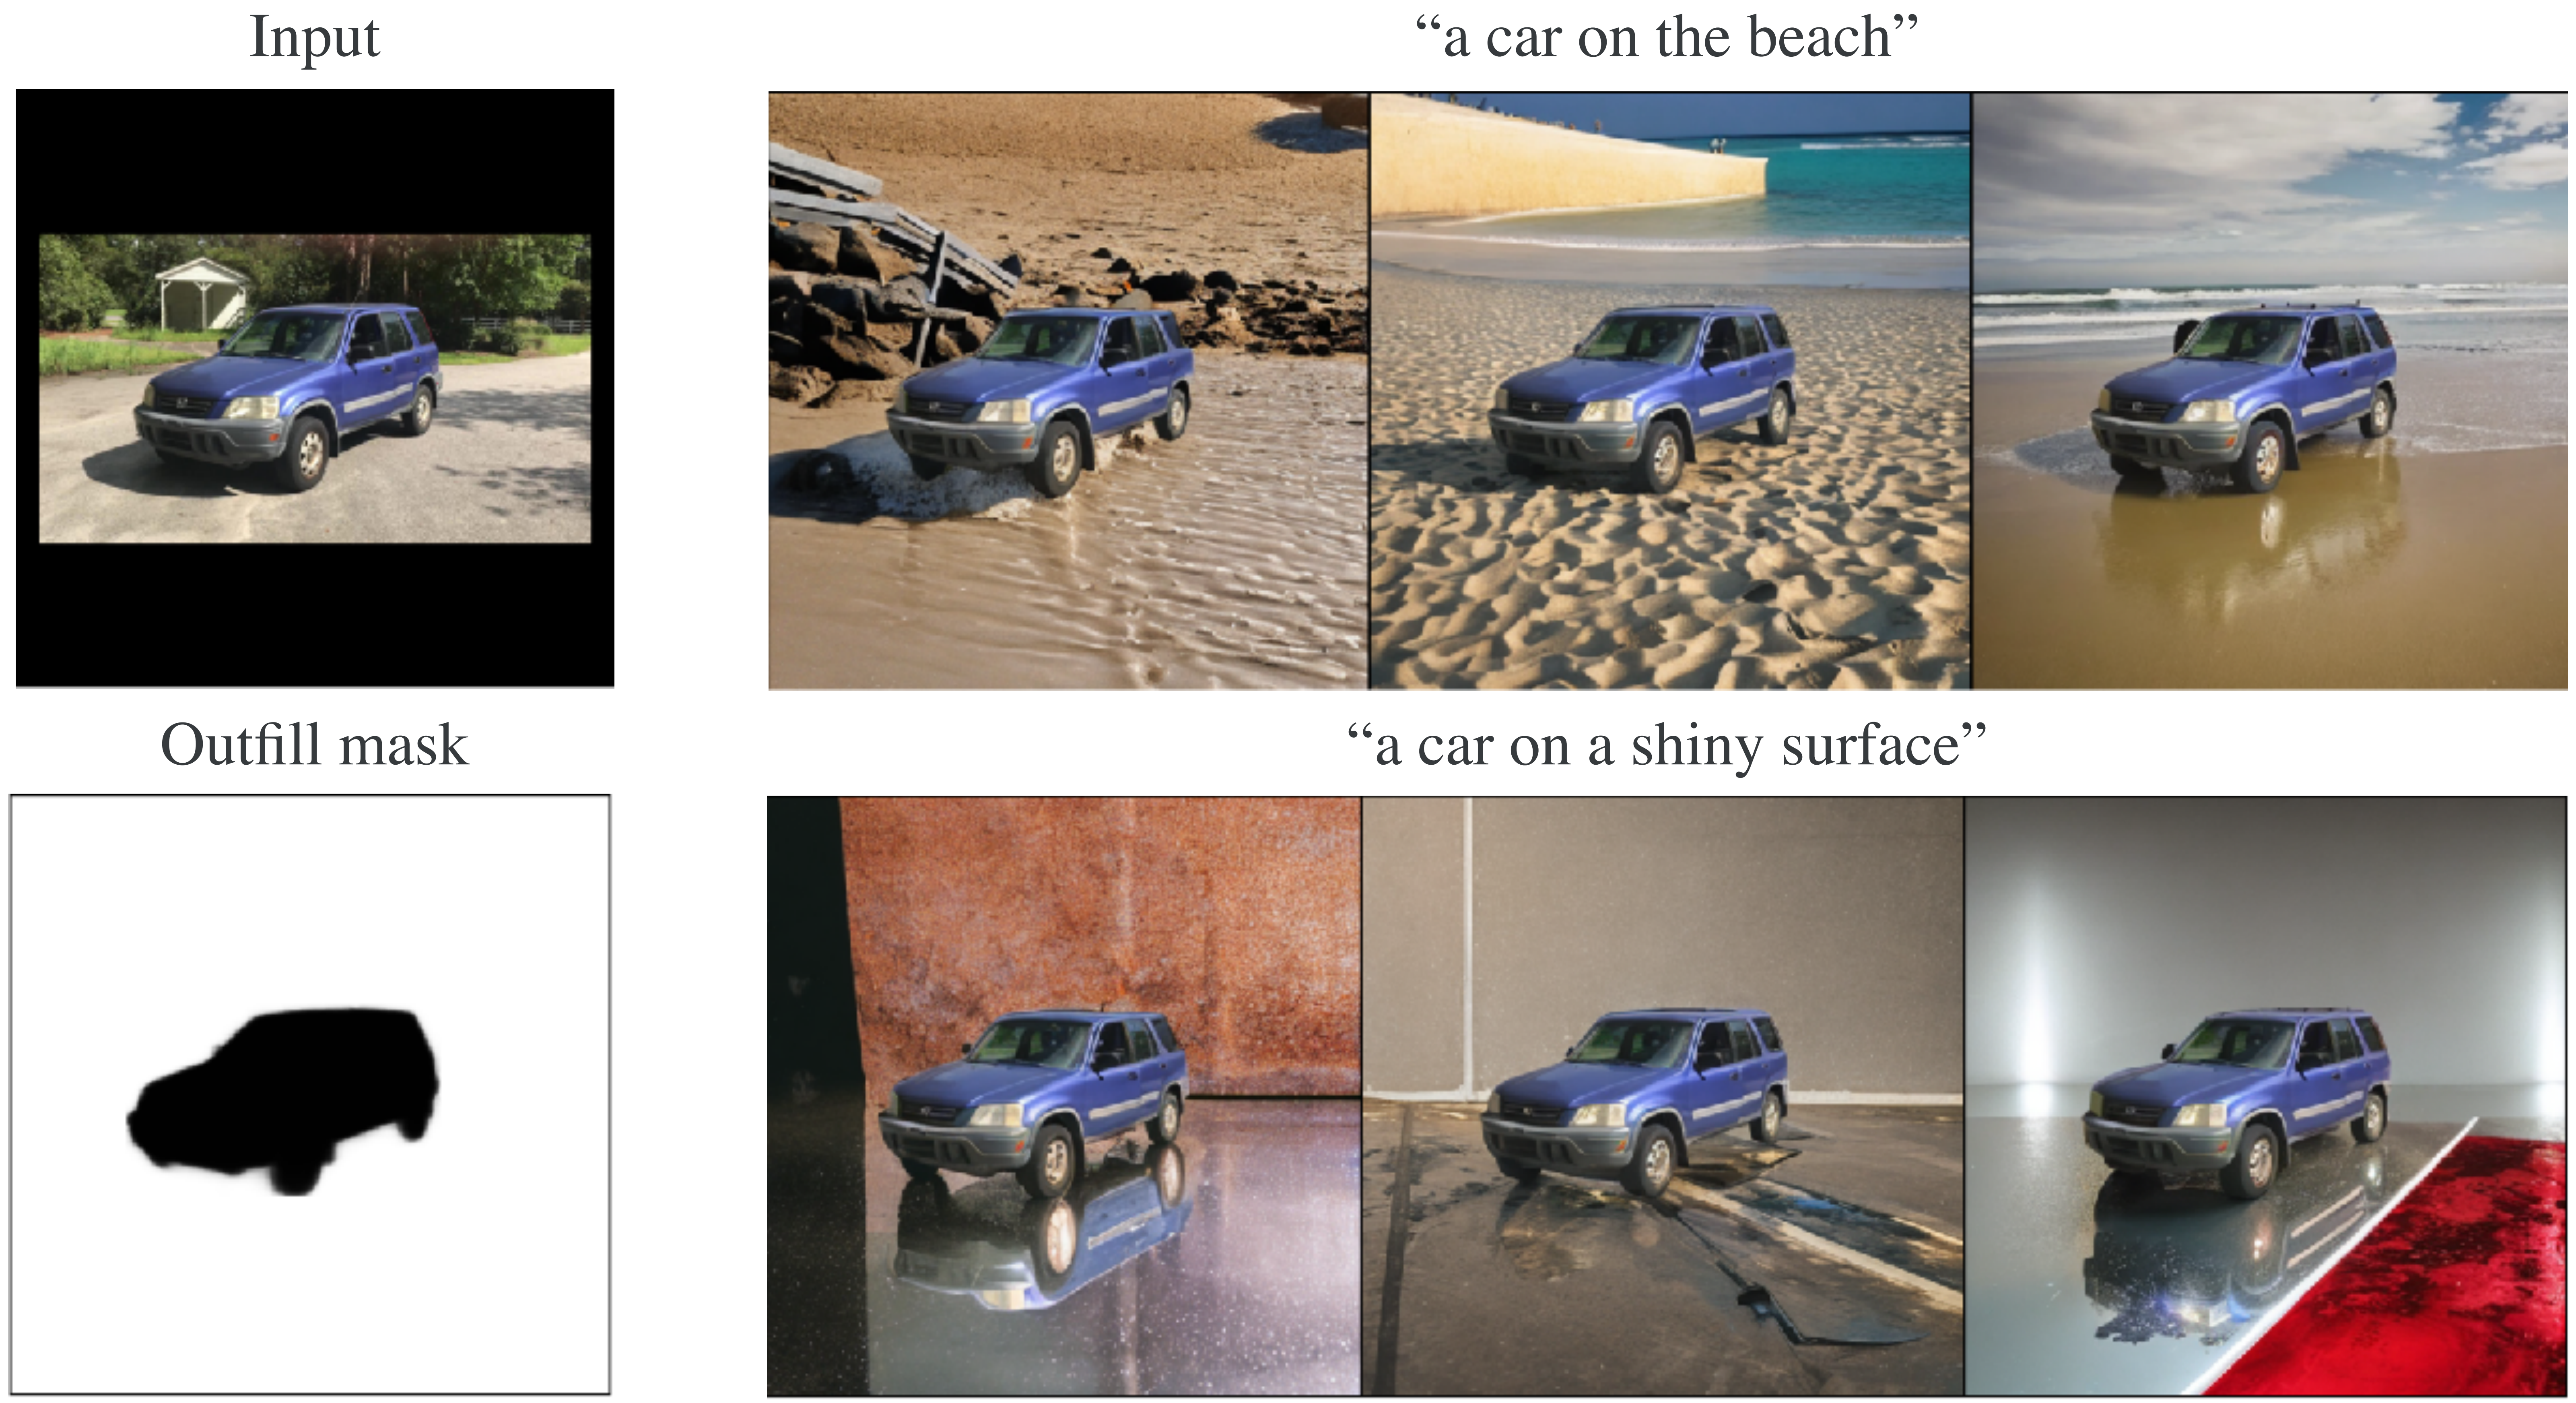


700

420

445

Ground truth

ViewNeTI prediction

Camera encoding freq $0.5 \Rightarrow 0.25$

Camera encoding freq $0.5 \Rightarrow 1$

No norm scaling

No augmentations

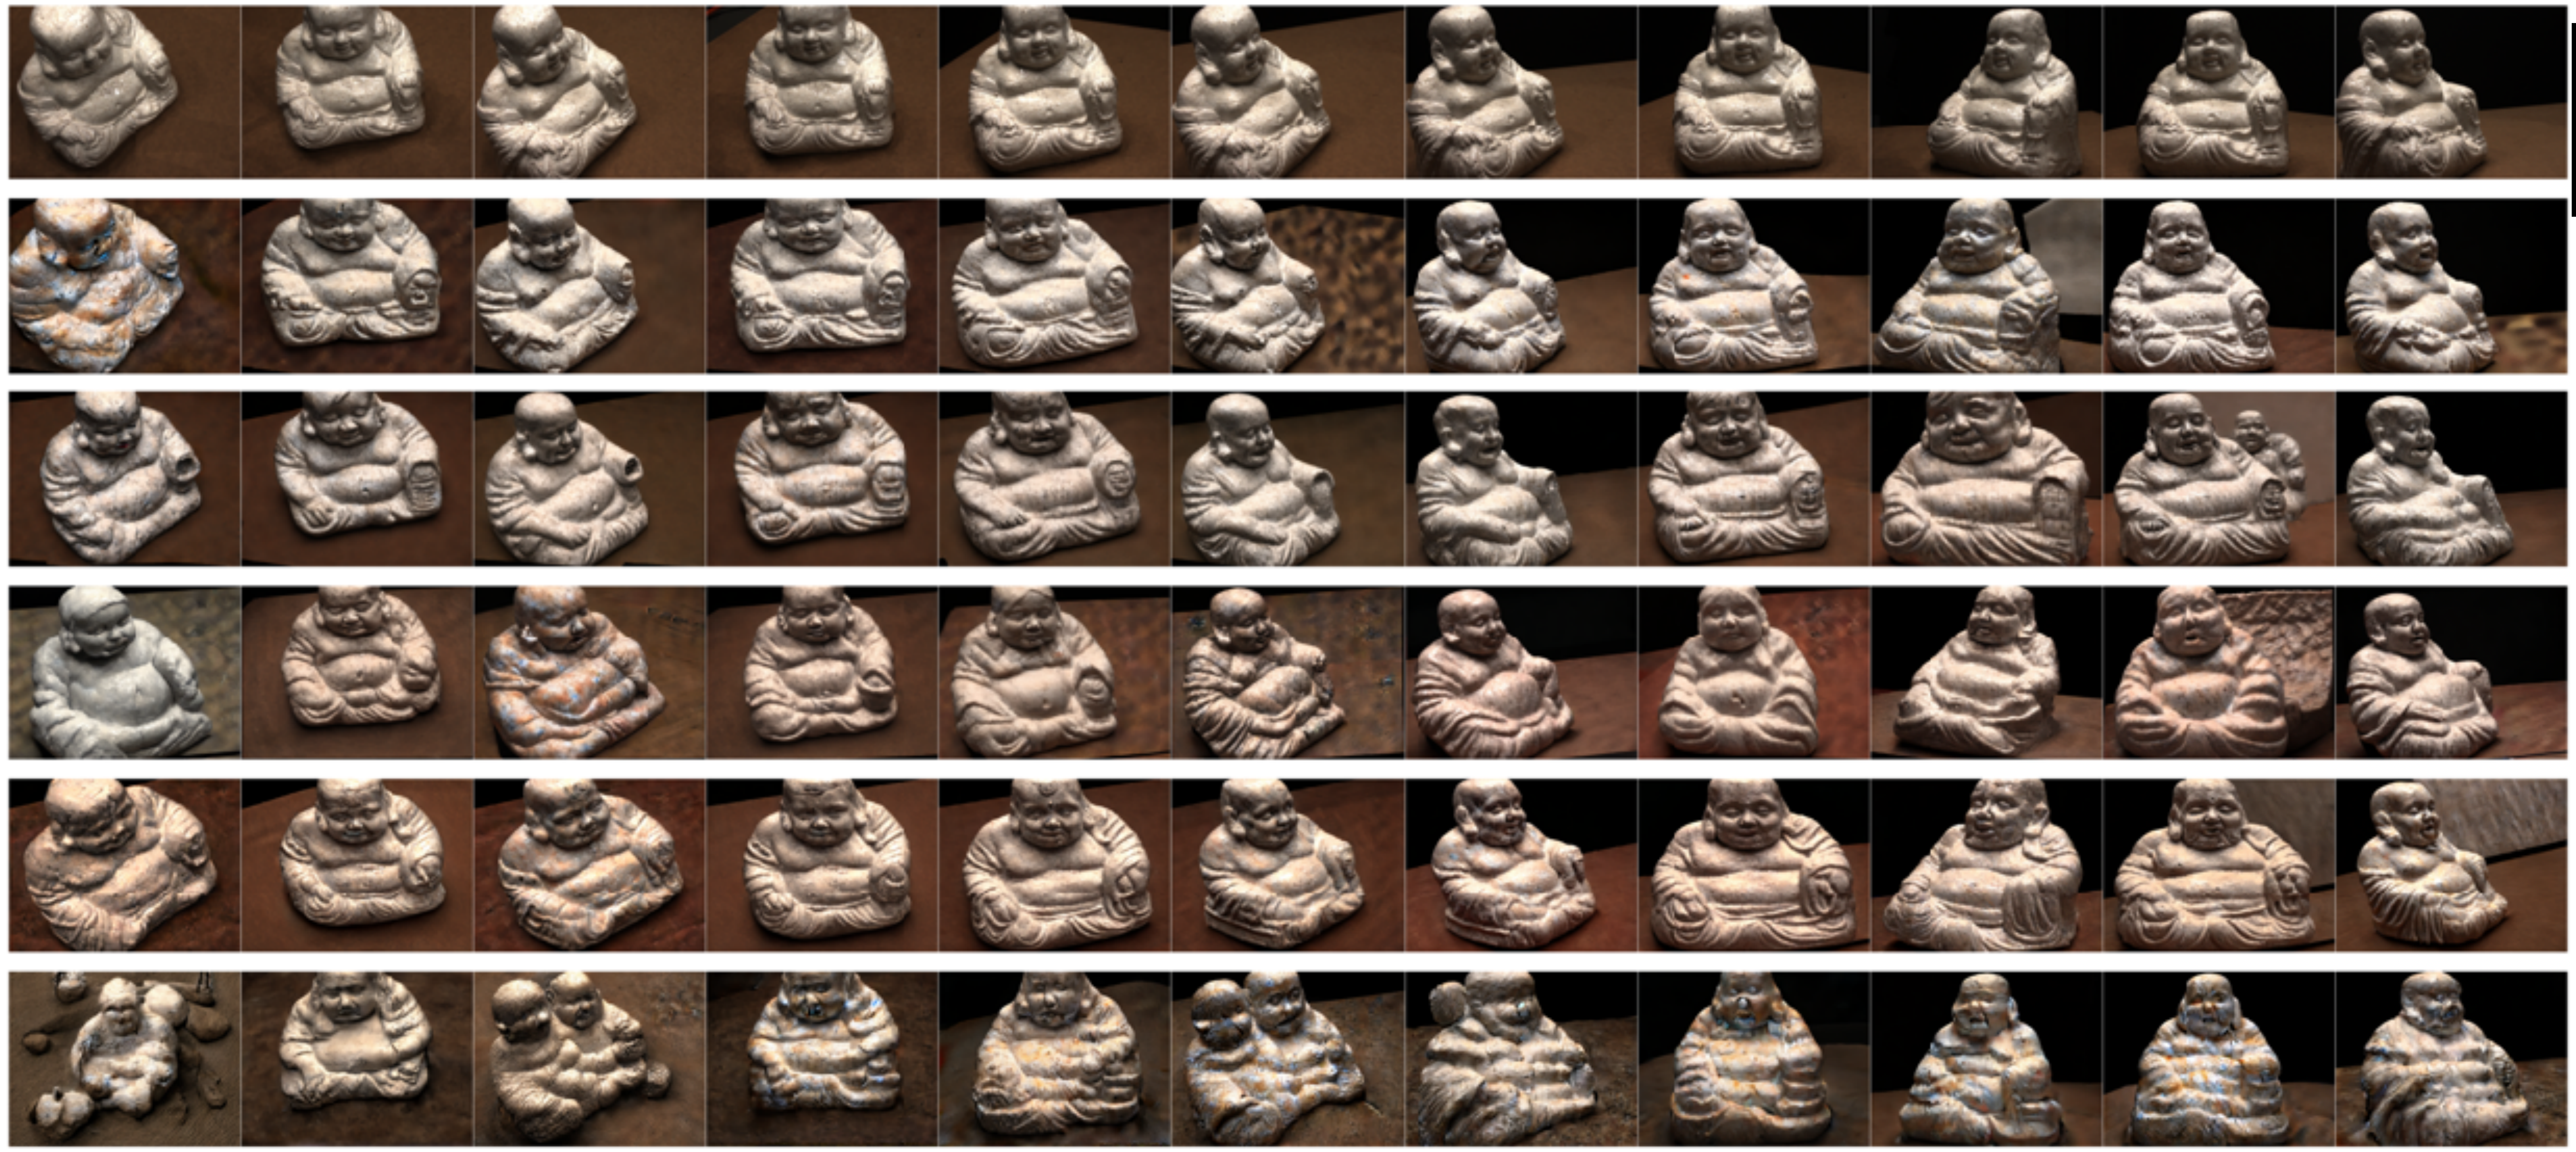

500

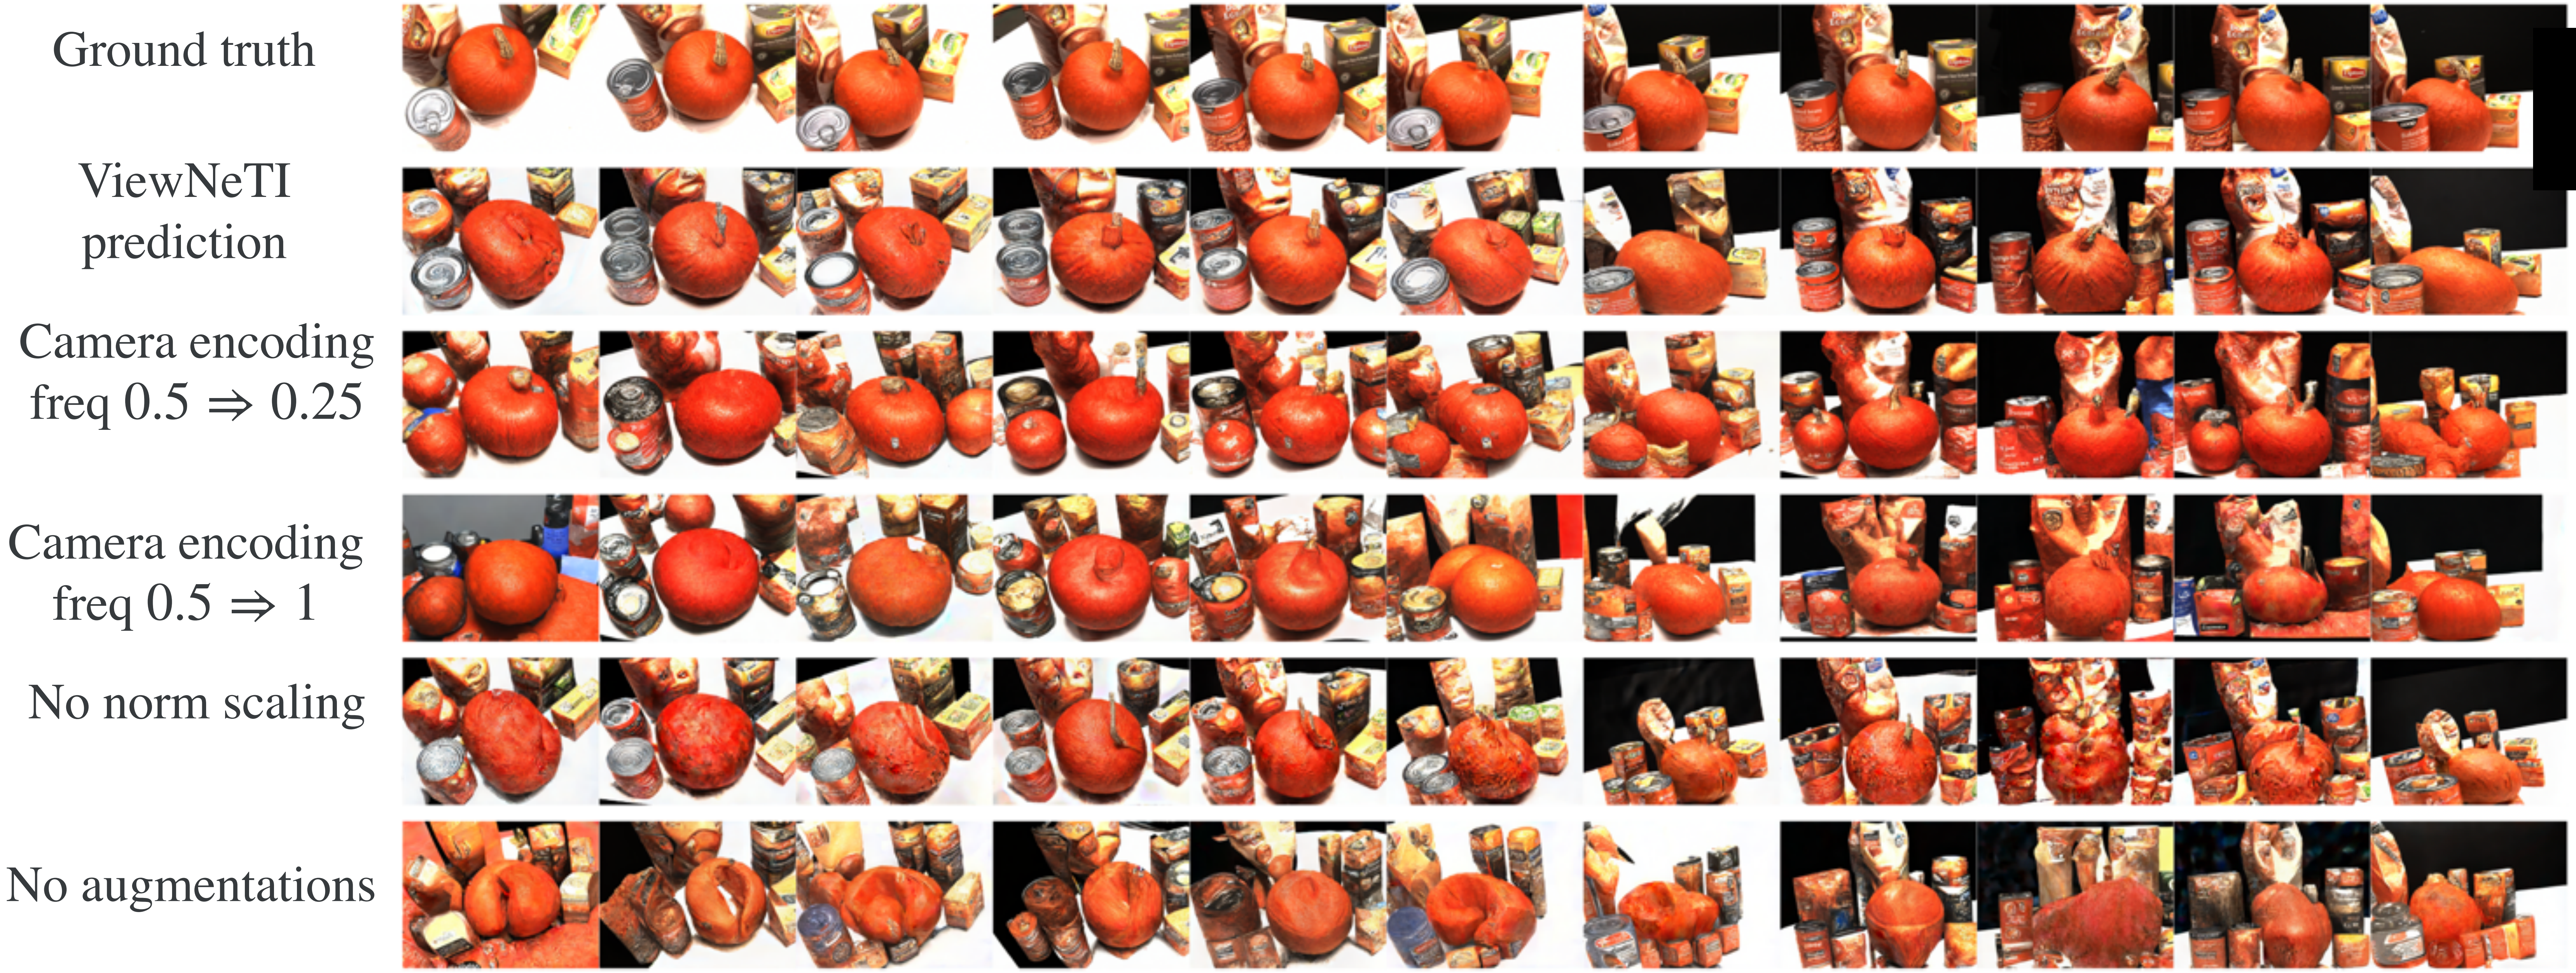
Ground truth
ViewNeTI prediction
Camera encoding freq 0.5 ⇒ 0.25
Camera encoding freq 0.5 ⇒ 1
No norm scaling
No augmentations

445

500

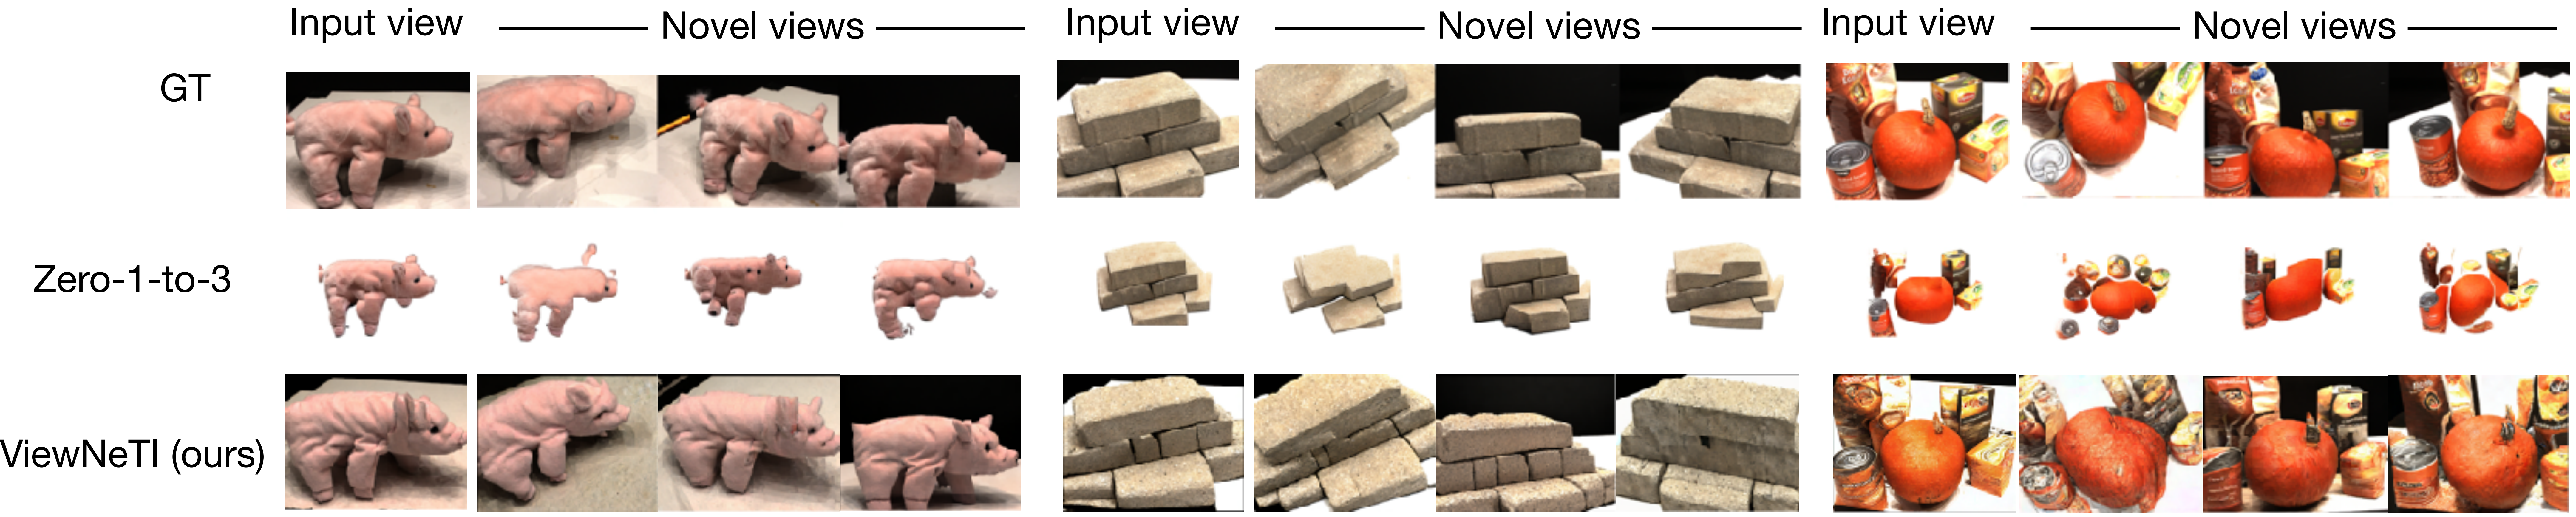
Input view
Novel views
Input view
Novel views
Input view
Novel views
GT
Zero-1-to-3
ViewNeTI (ours)

290

740

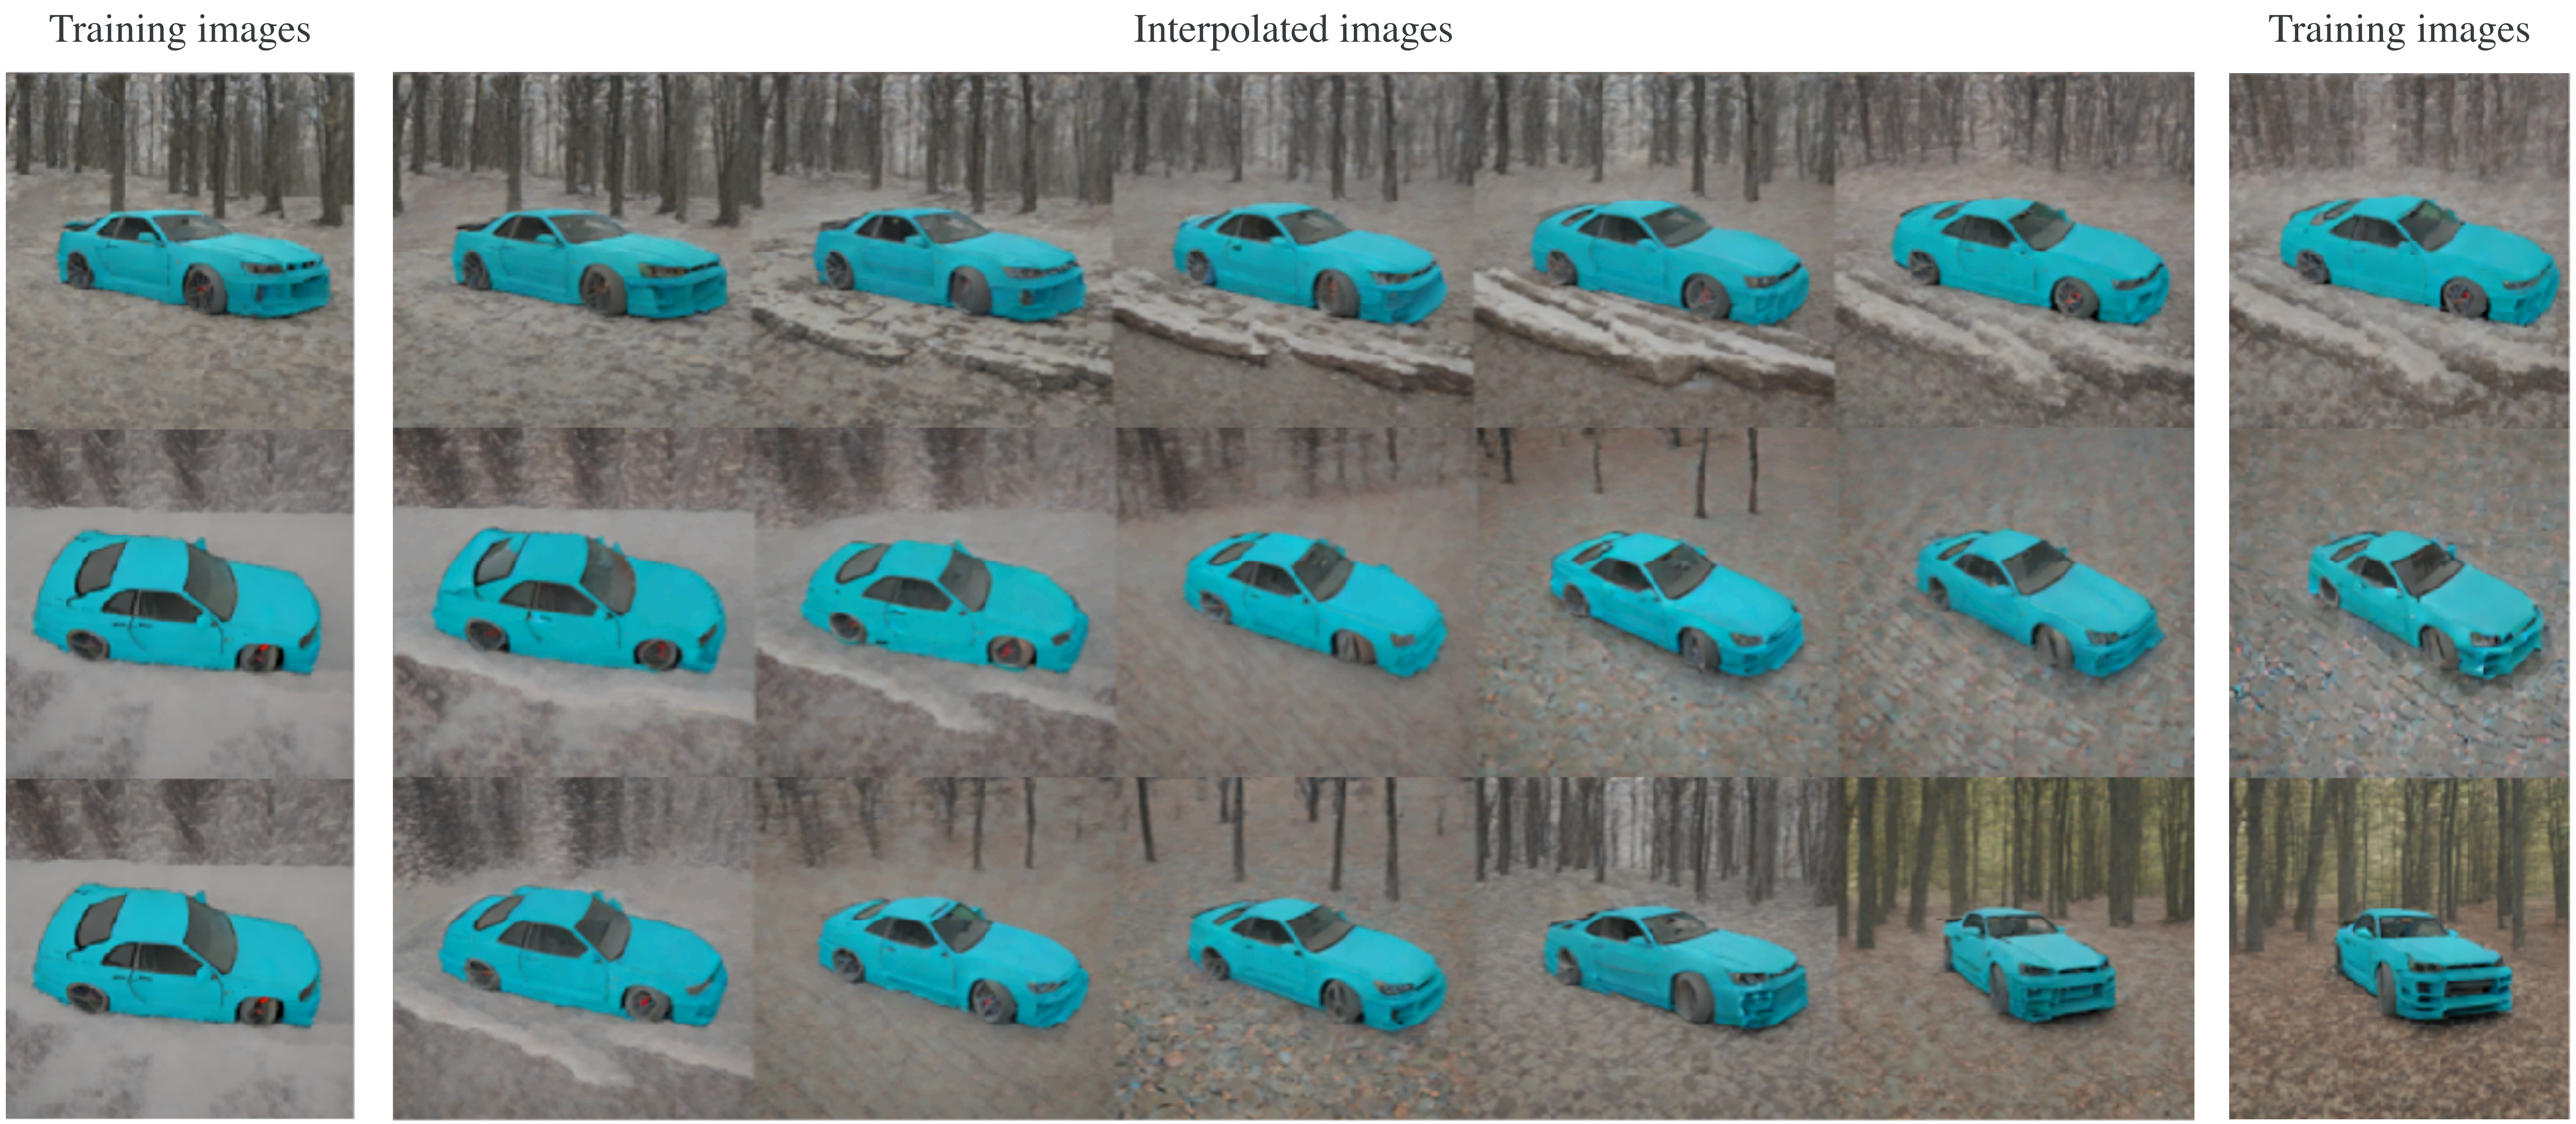


235

340

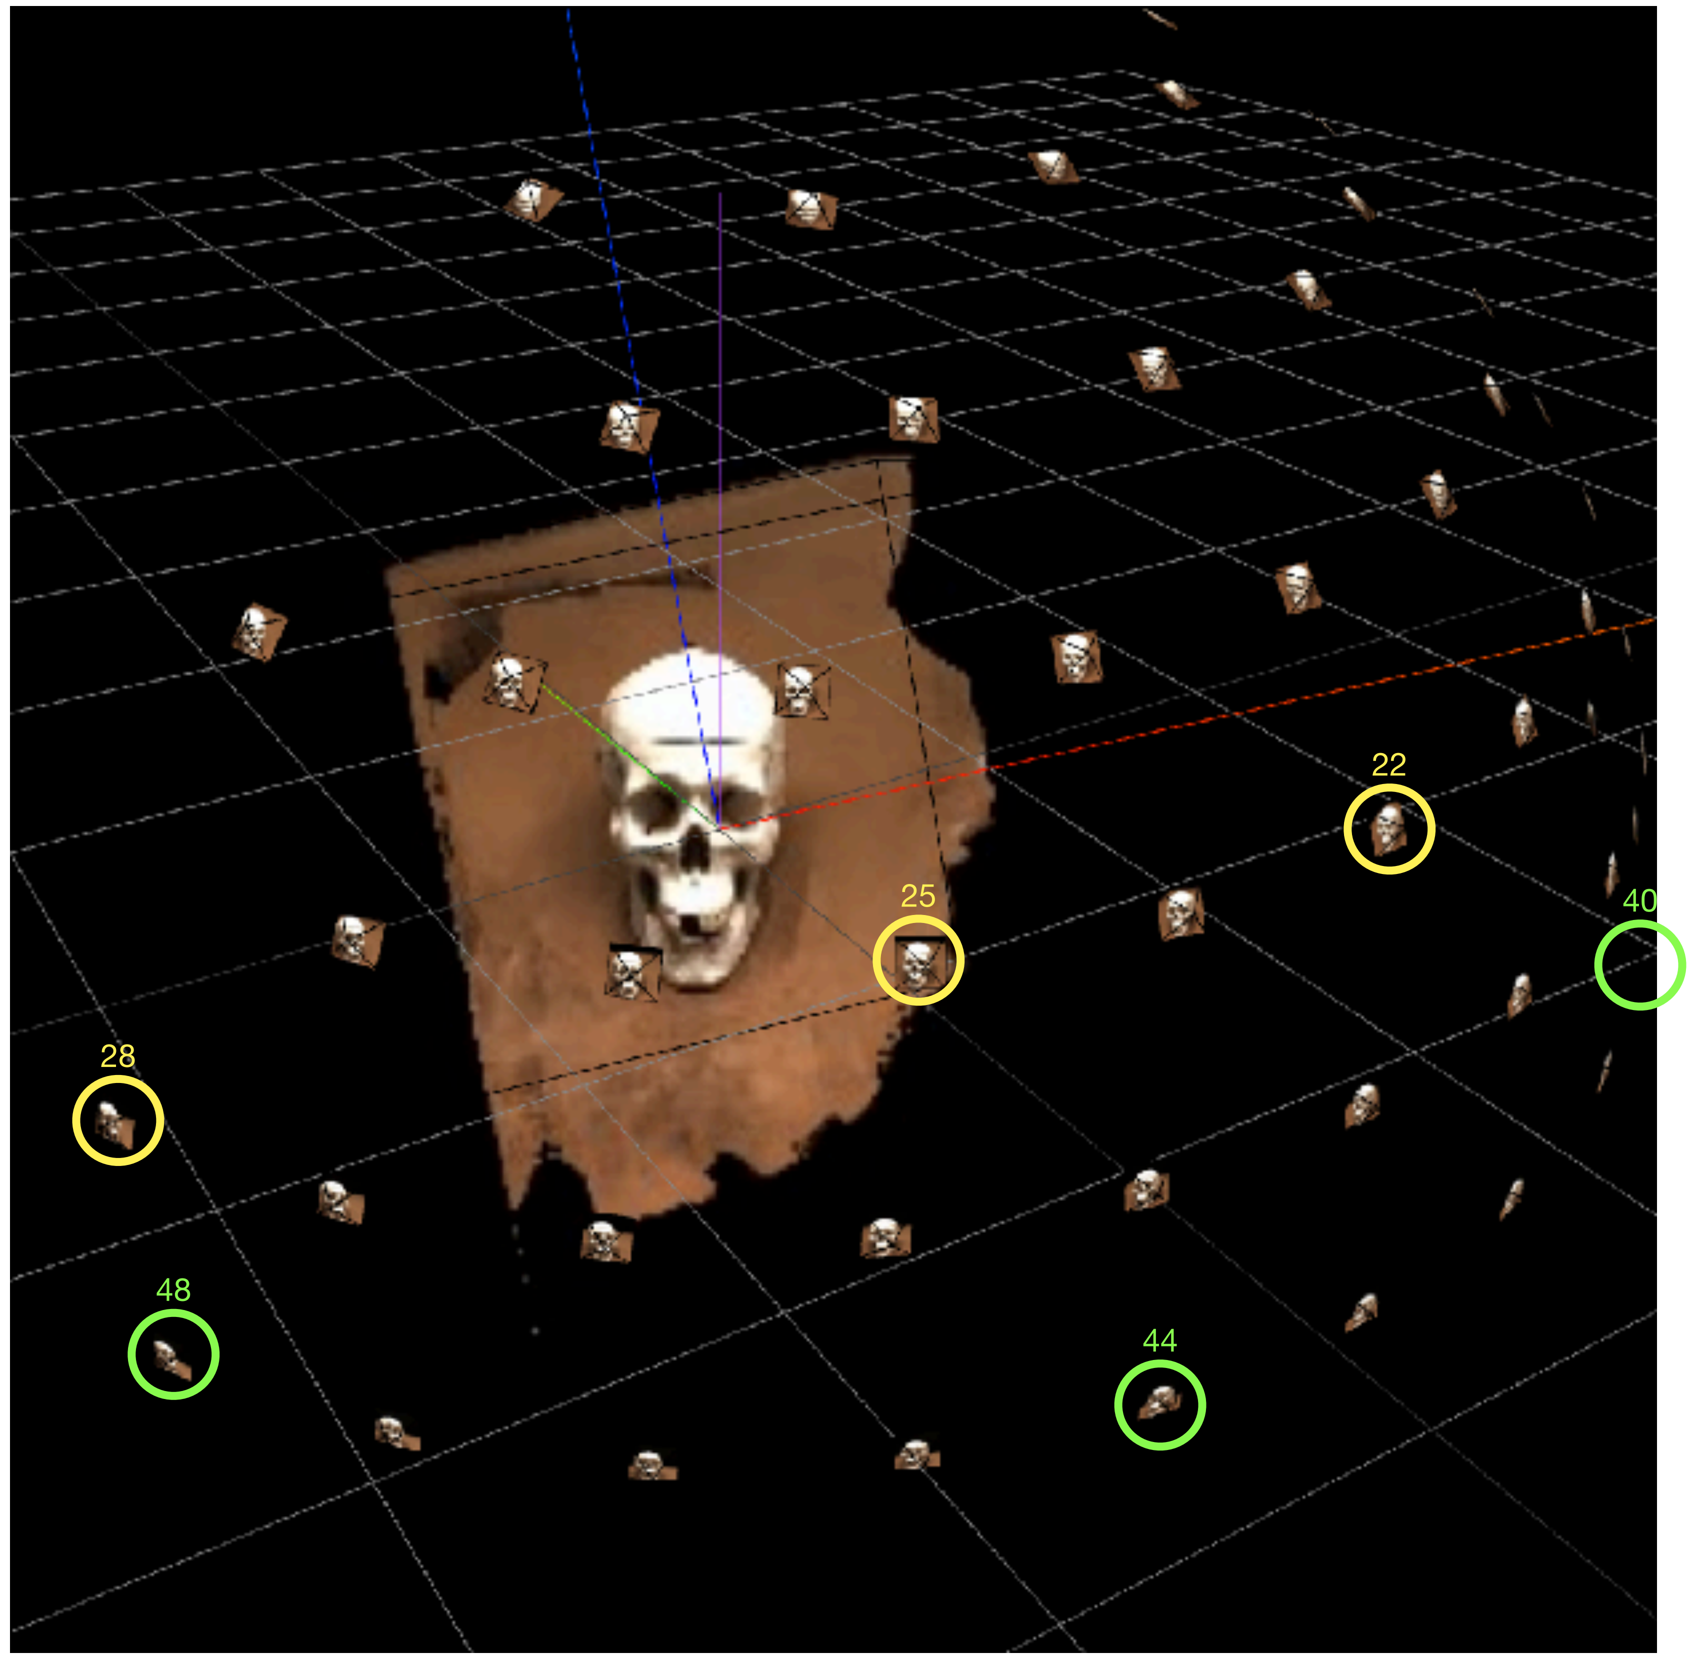


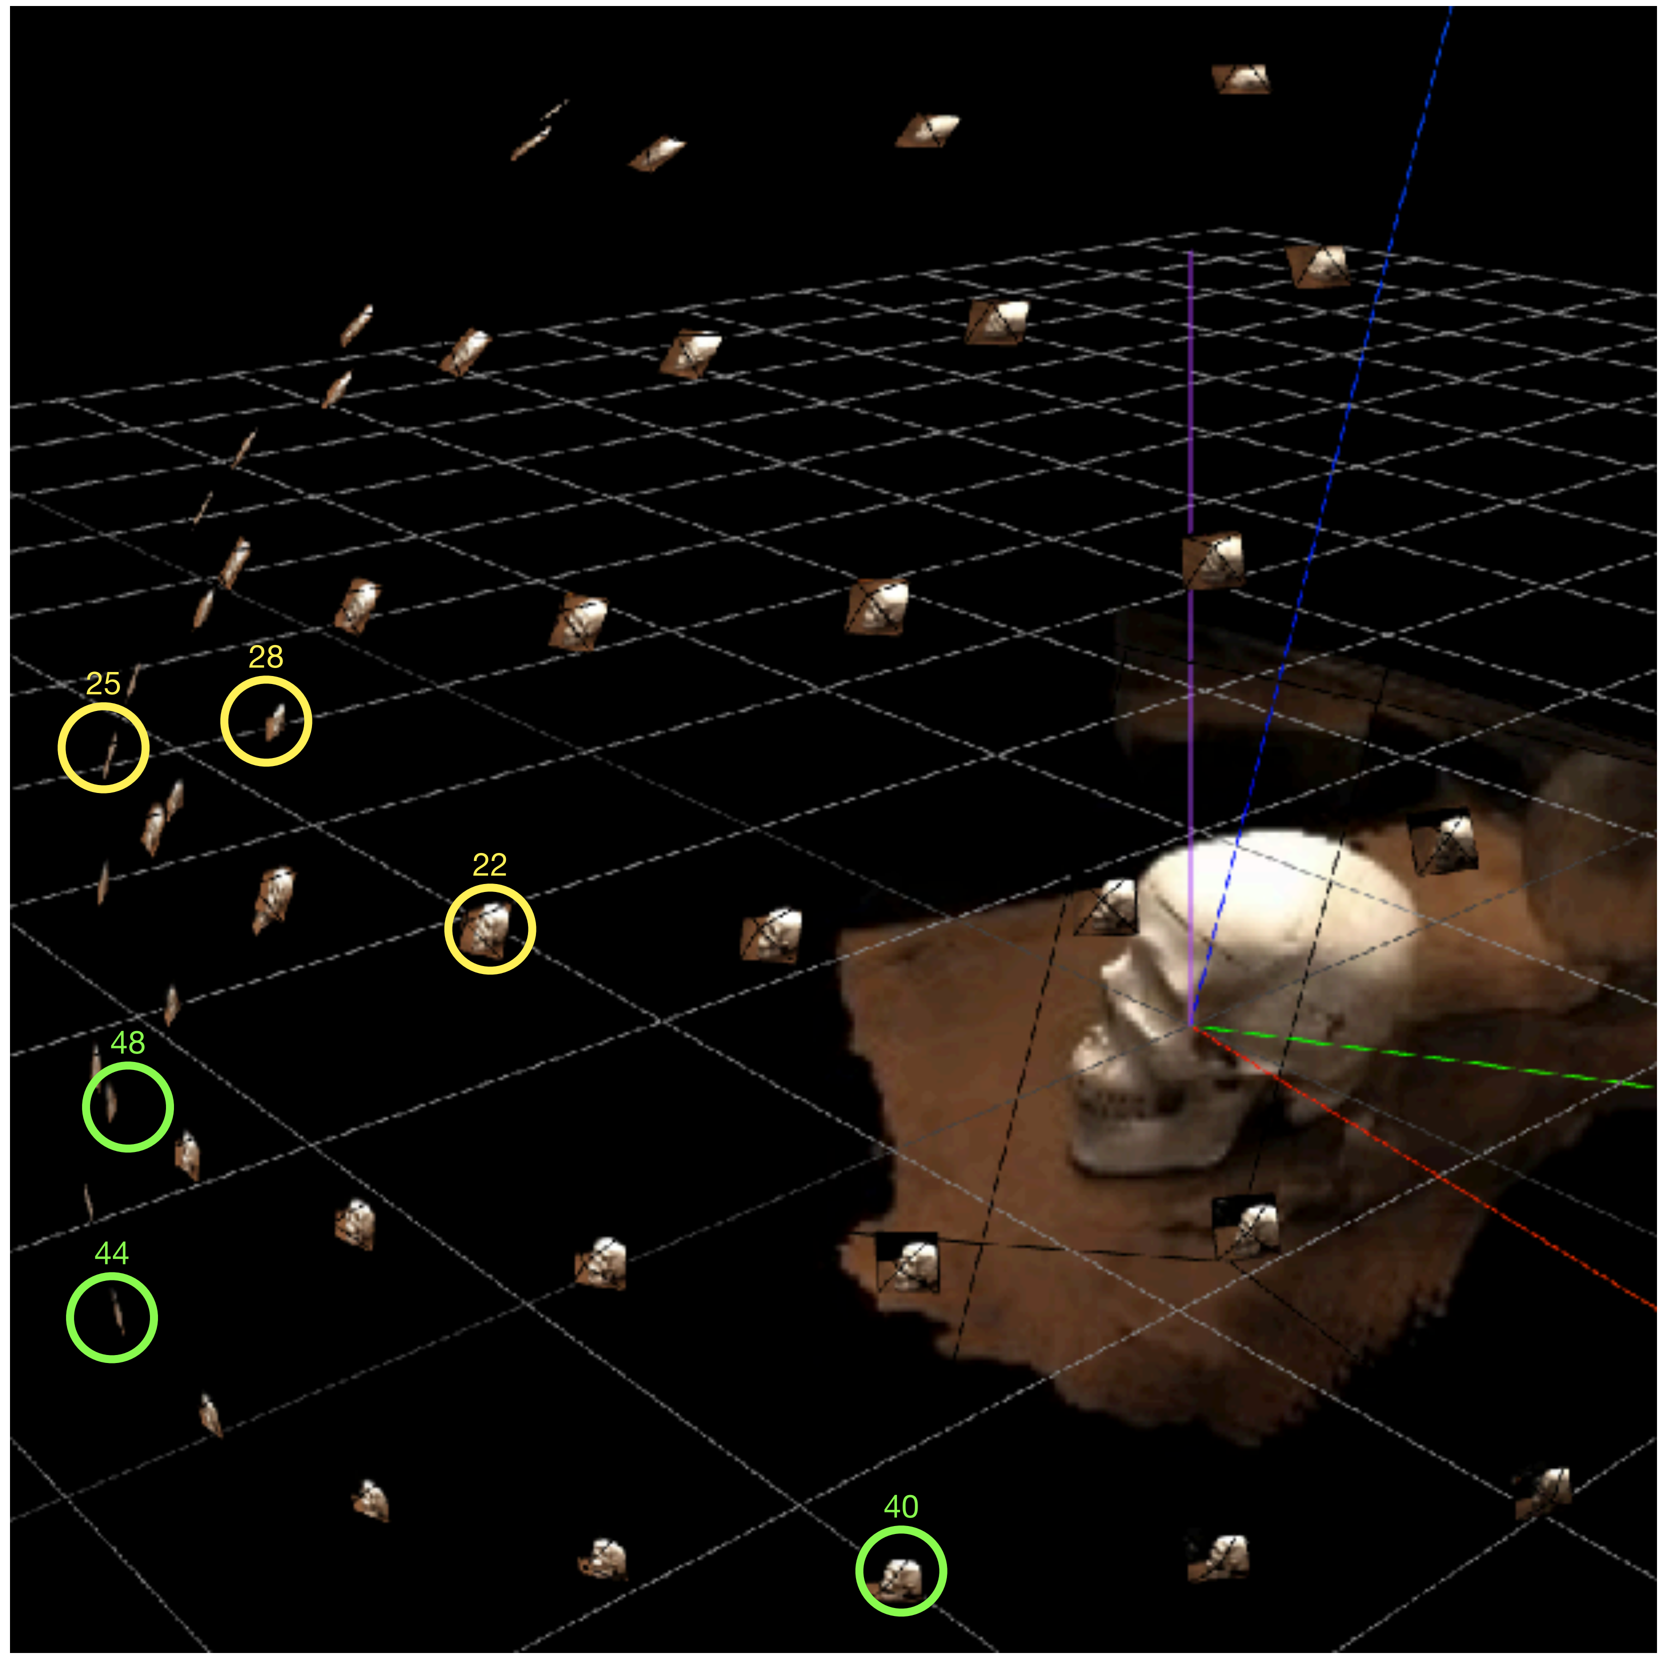


550

435

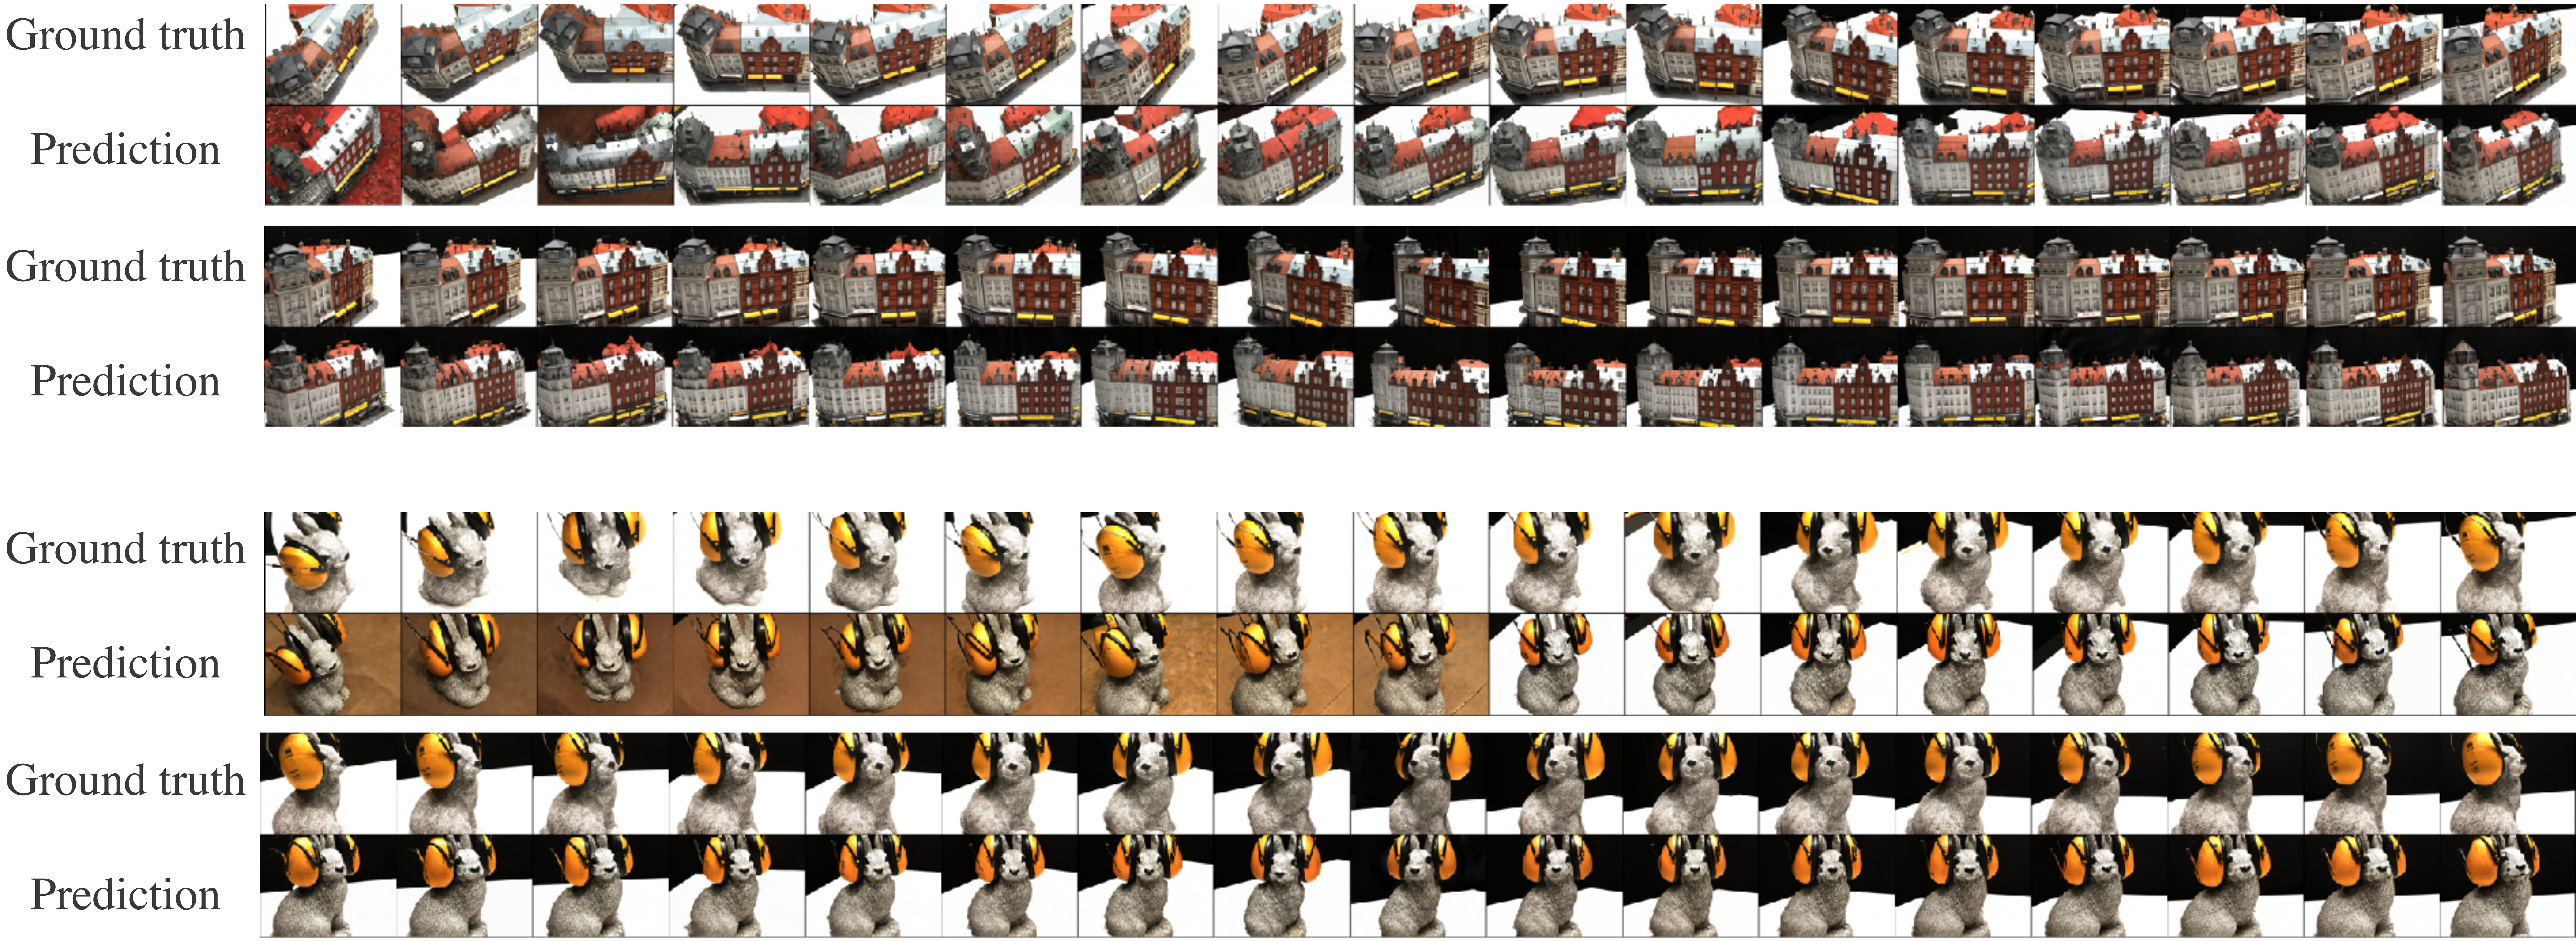
Ground truth
Prediction
Ground truth
Prediction
Ground truth
Prediction
Ground truth
Prediction

360

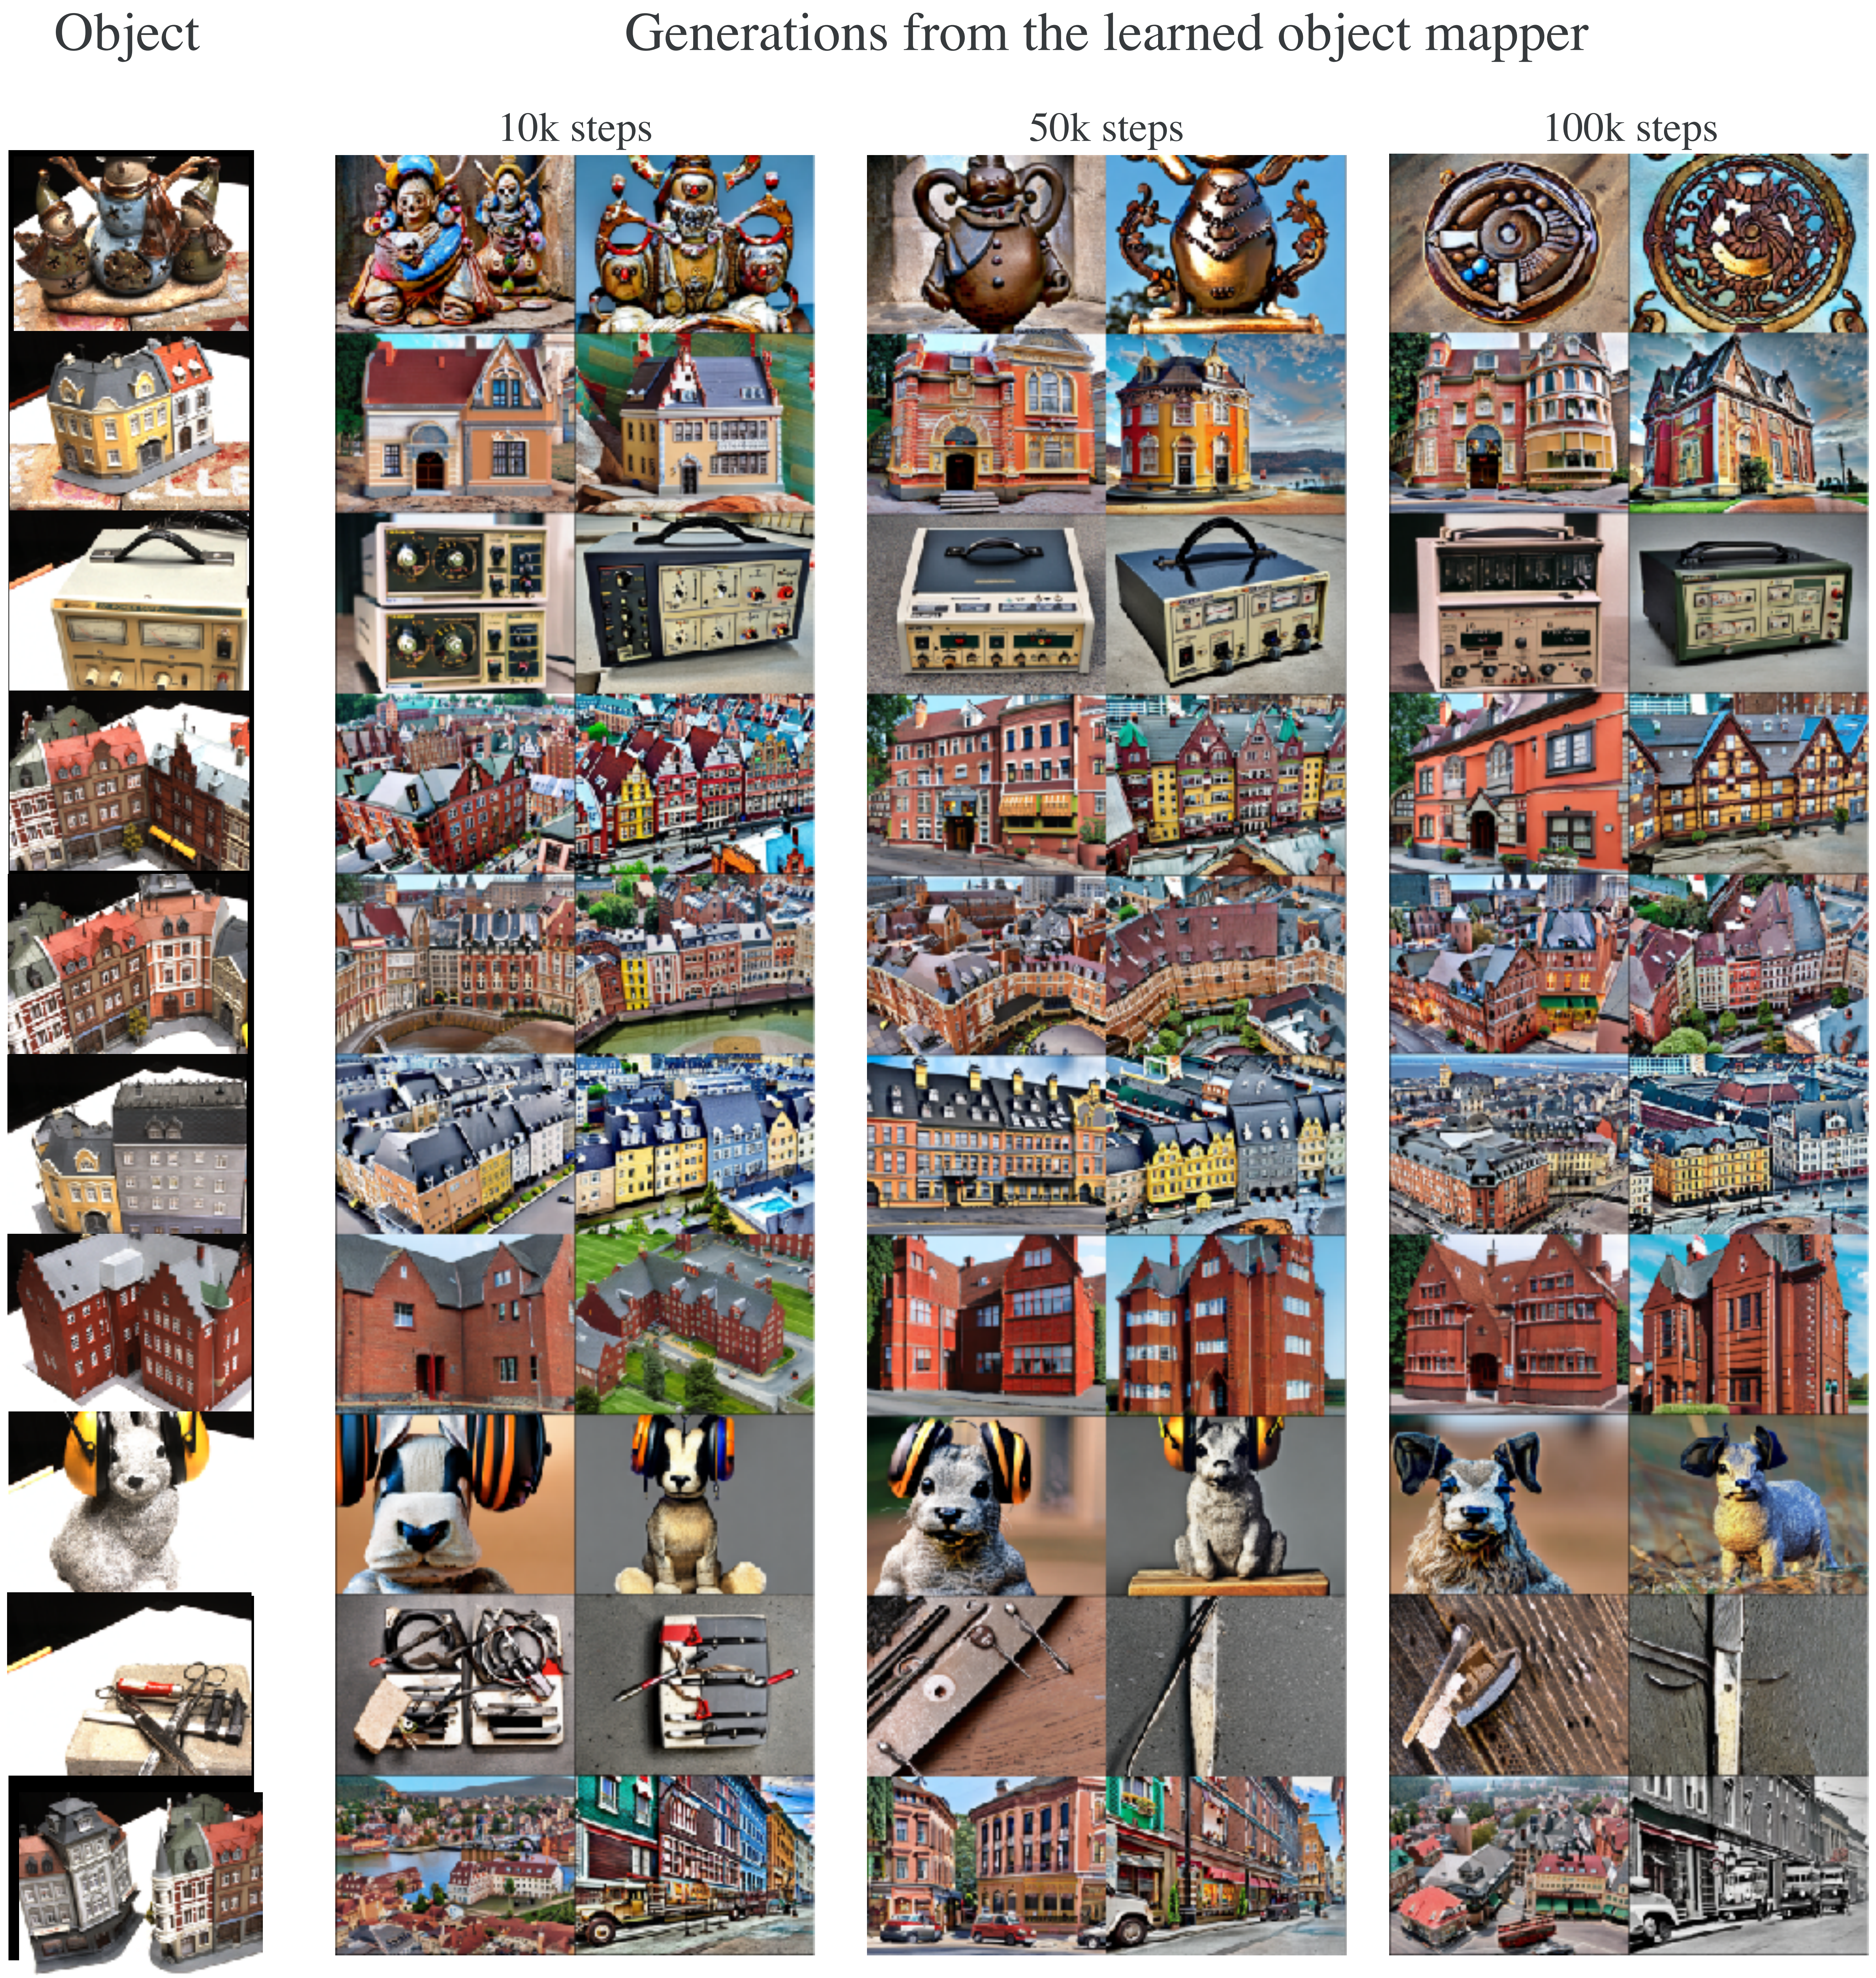
Object
Generations from the learned object mapper
10k steps
50k steps
100k steps

890

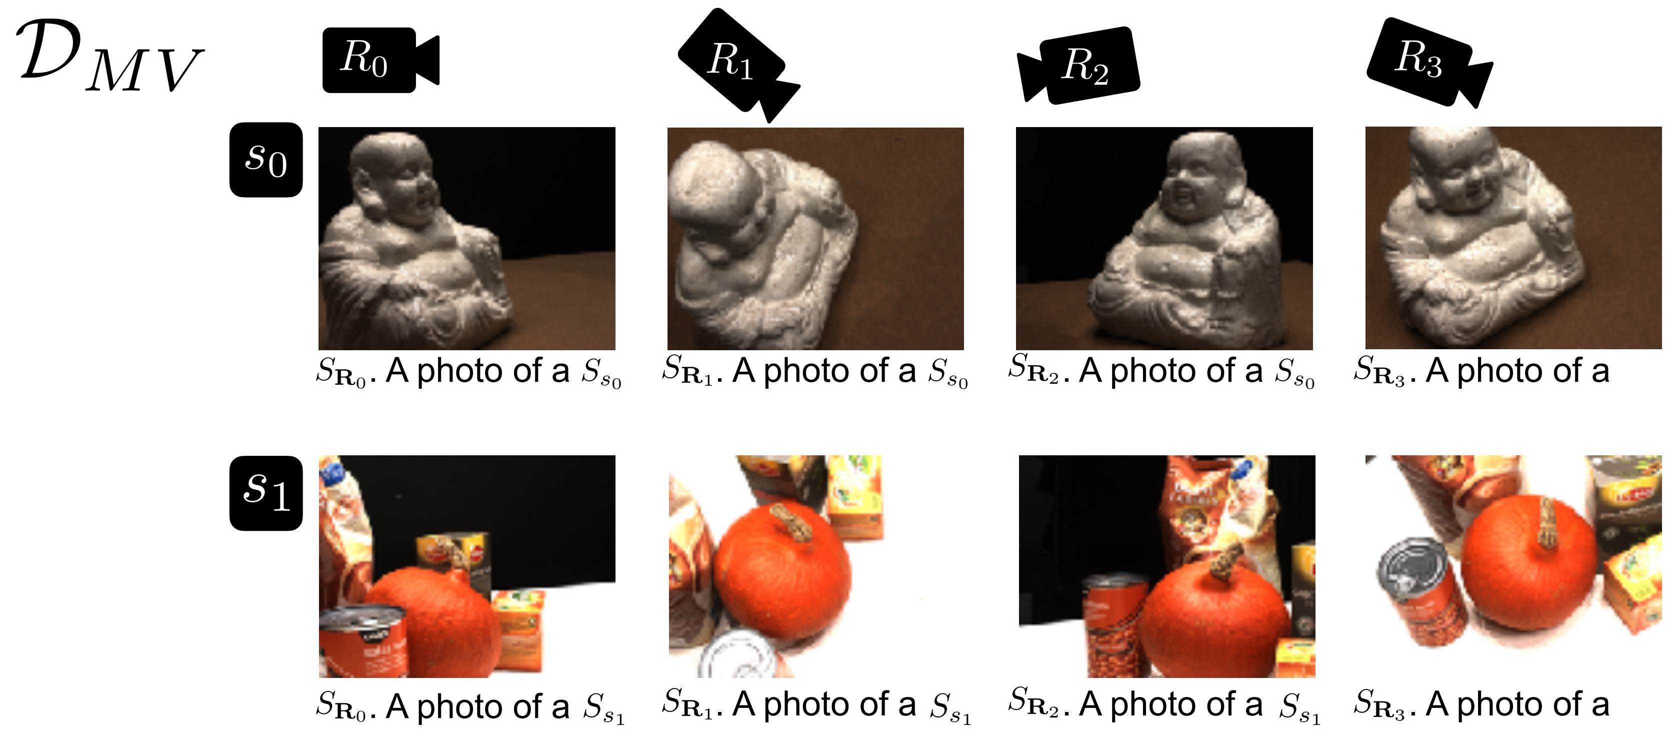

$\mathcal{D}_{MV}$
$R_0$
$R_1$
$R_2$
$R_3$
$s_0$
$S_{\mathbf{R}_0}$. A photo of a $S_{s_0}$
$S_{\mathbf{R}_1}$. A photo of a $S_{s_0}$
$S_{\mathbf{R}_2}$. A photo of a $S_{s_0}$
$S_{\mathbf{R}_3}$. A photo of a
$s_1$
$S_{\mathbf{R}_0}$. A photo of a $S_{s_1}$
$S_{\mathbf{R}_1}$. A photo of a $S_{s_1}$
$S_{\mathbf{R}_2}$. A photo of a $S_{s_1}$
$S_{\mathbf{R}_3}$. A photo of a


1200

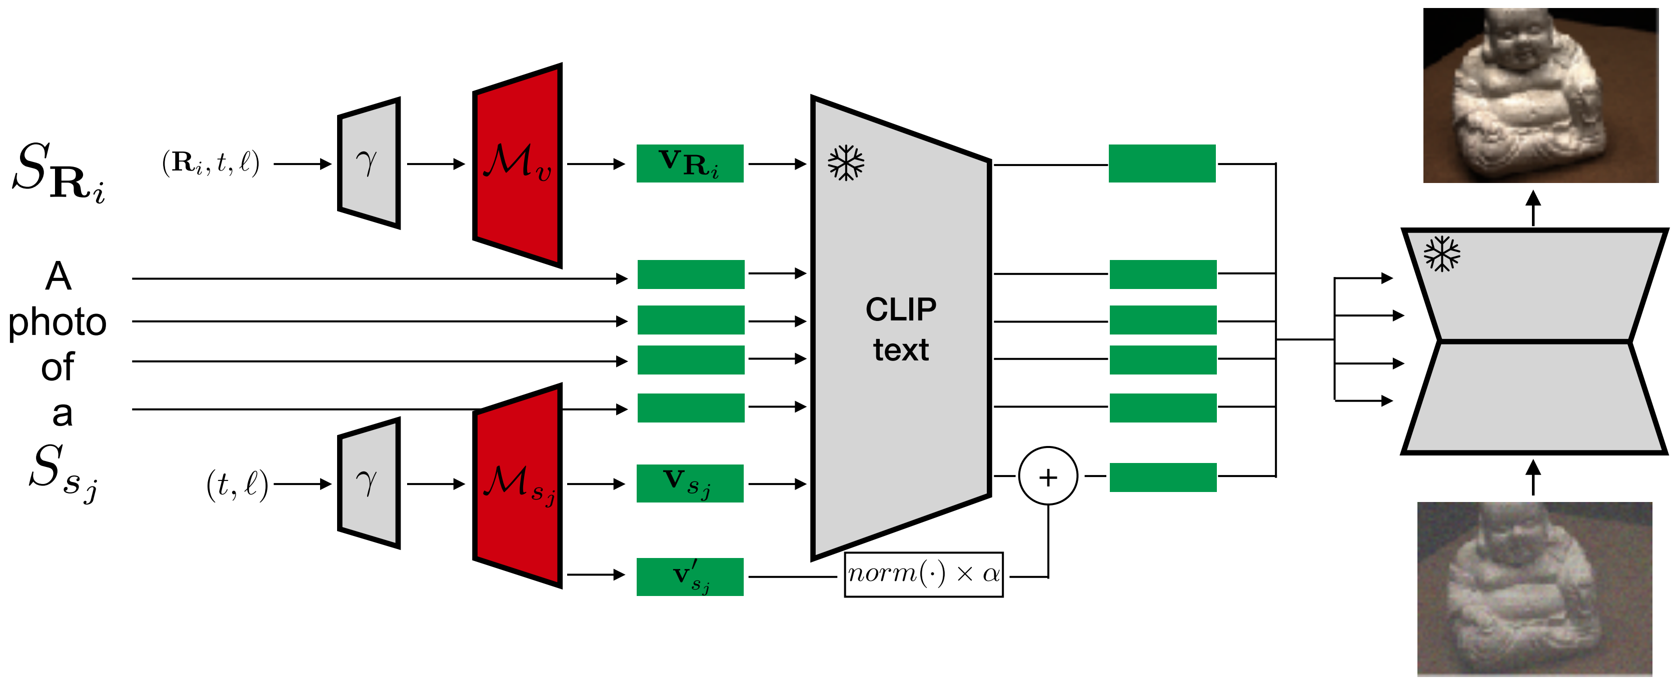

$S_{\mathbf{R}_i}$
$(\mathbf{R}_i, t, \ell)$
$\gamma$
$\mathcal{M}_v$
$\mathbf{v}_{\mathbf{R}_i}$
A
photo
of
a
$S_{s_j}$
$(t, \ell)$
$\mathcal{M}_{s_j}$
$\mathbf{v}_{s_j}$
$\mathbf{v}'_{s_j}$
CLIP
text
$norm(\cdot) \times \alpha$


480

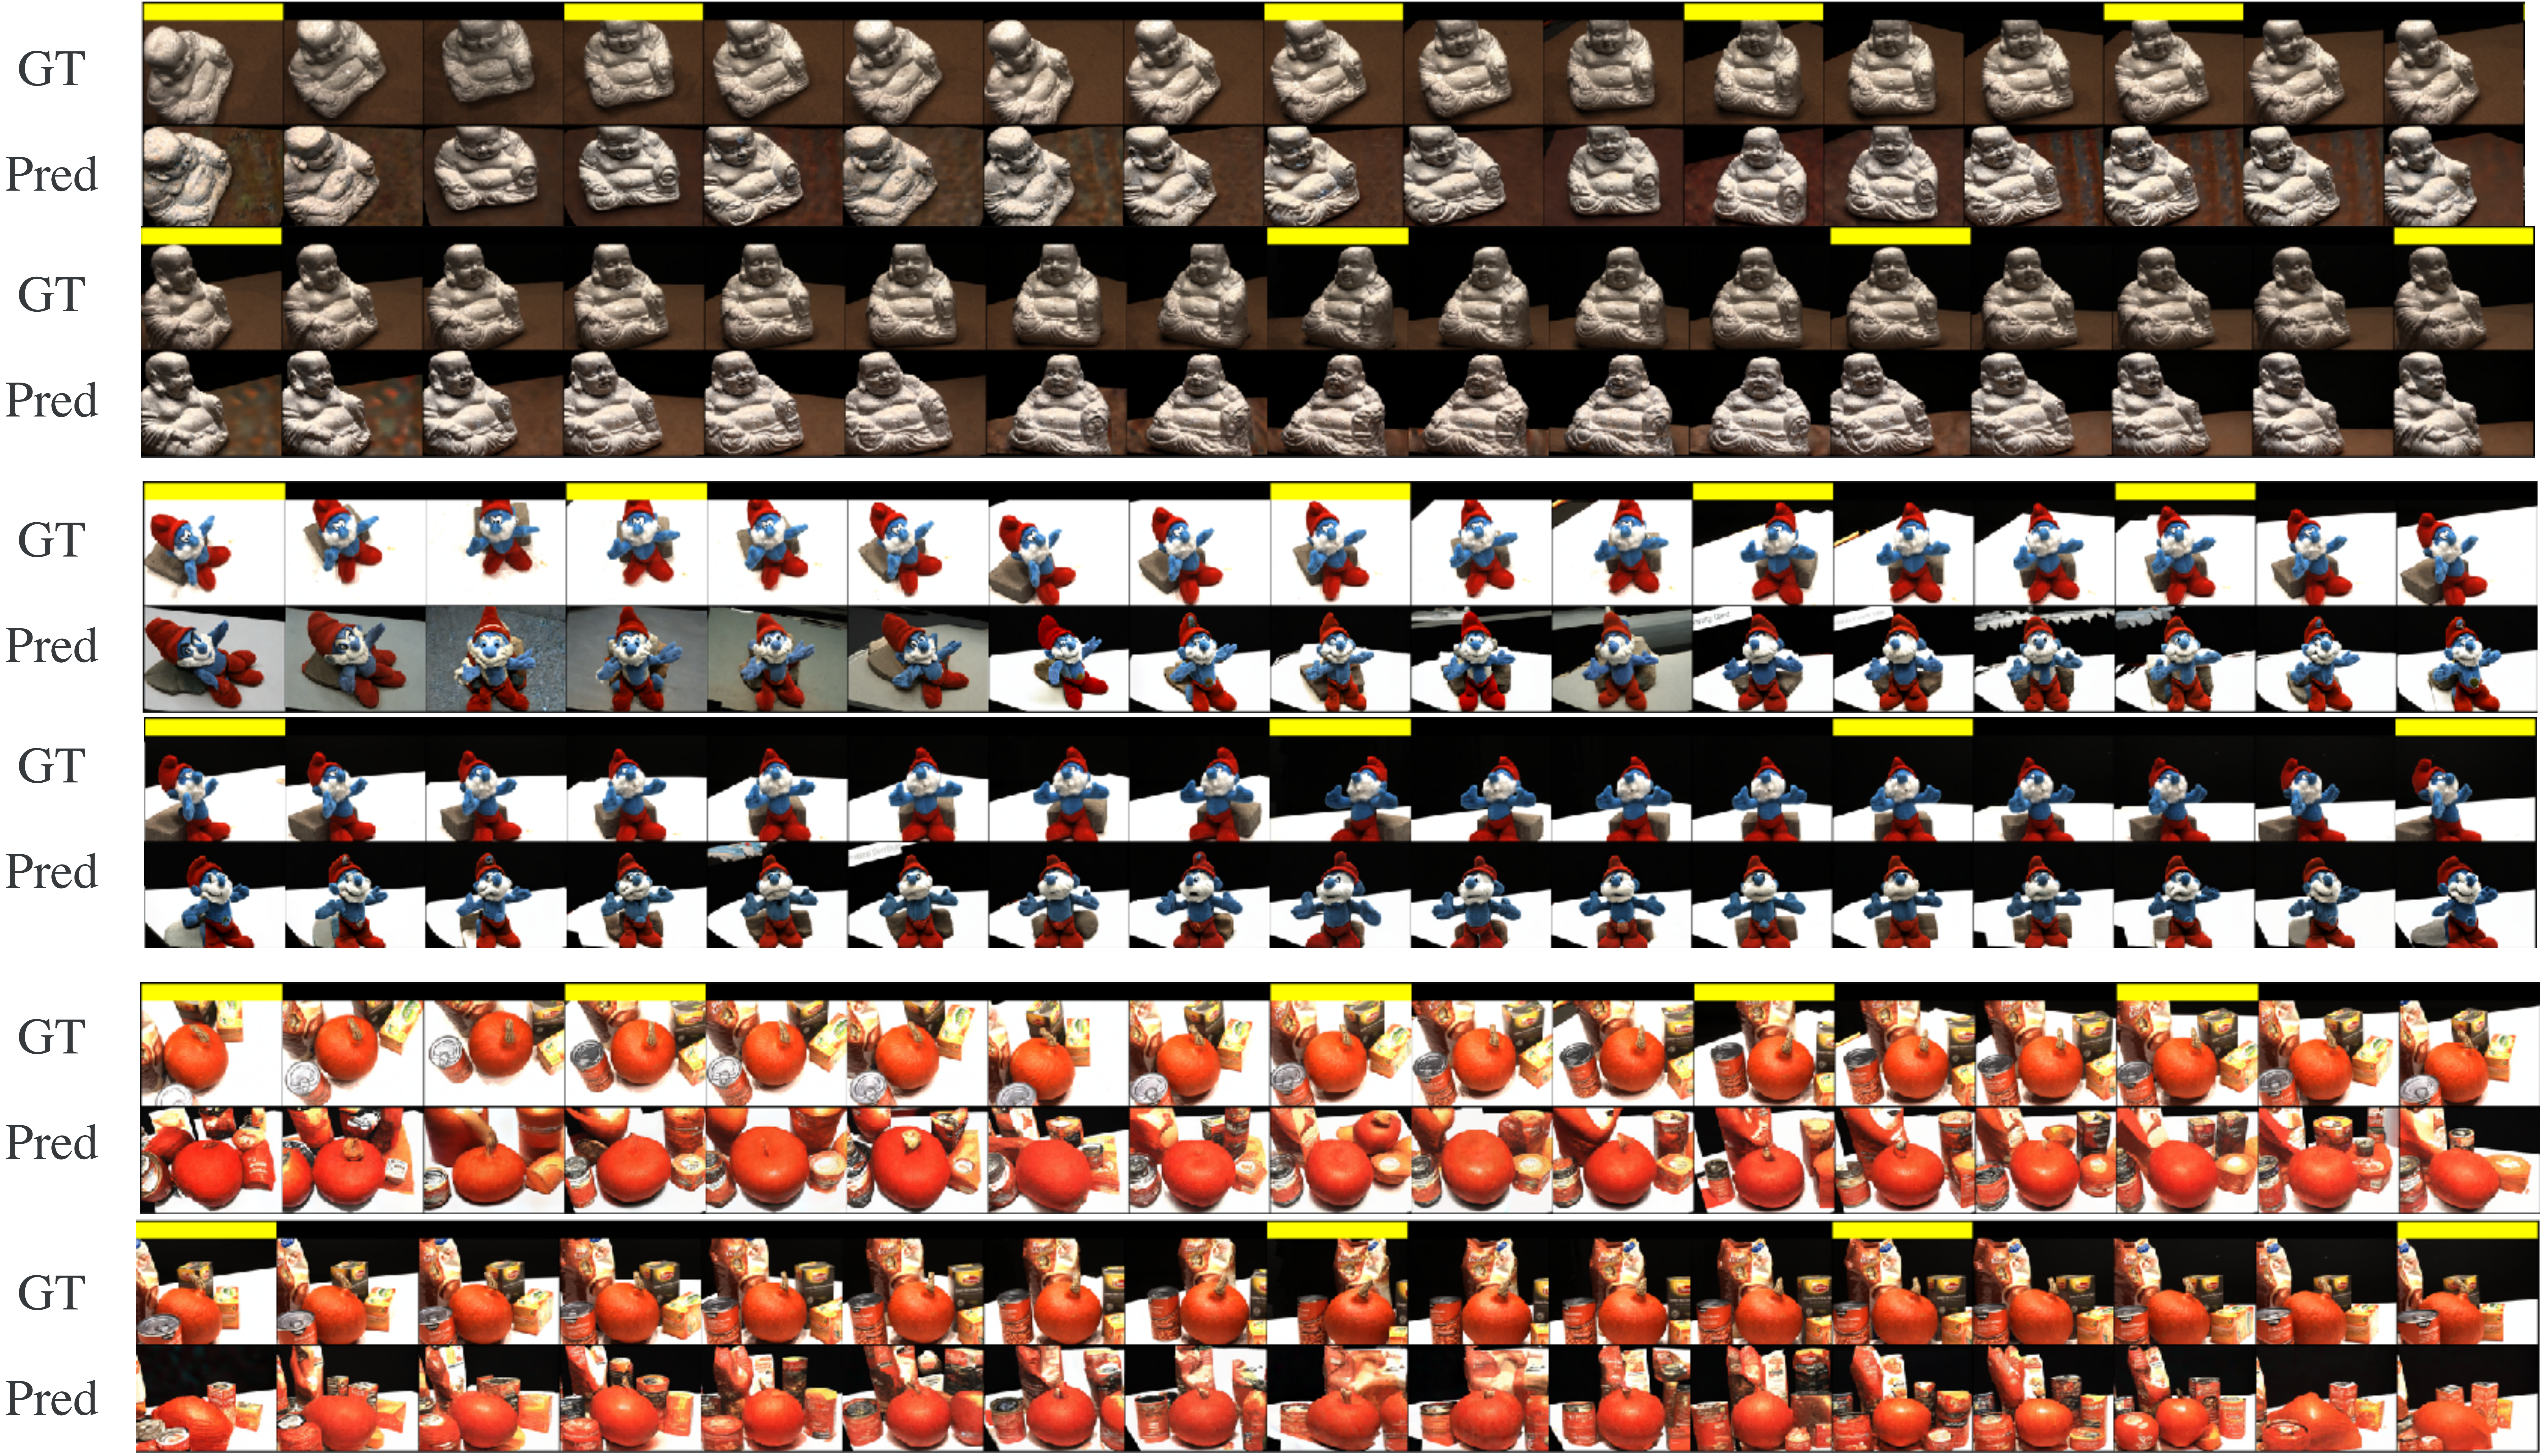


215

100

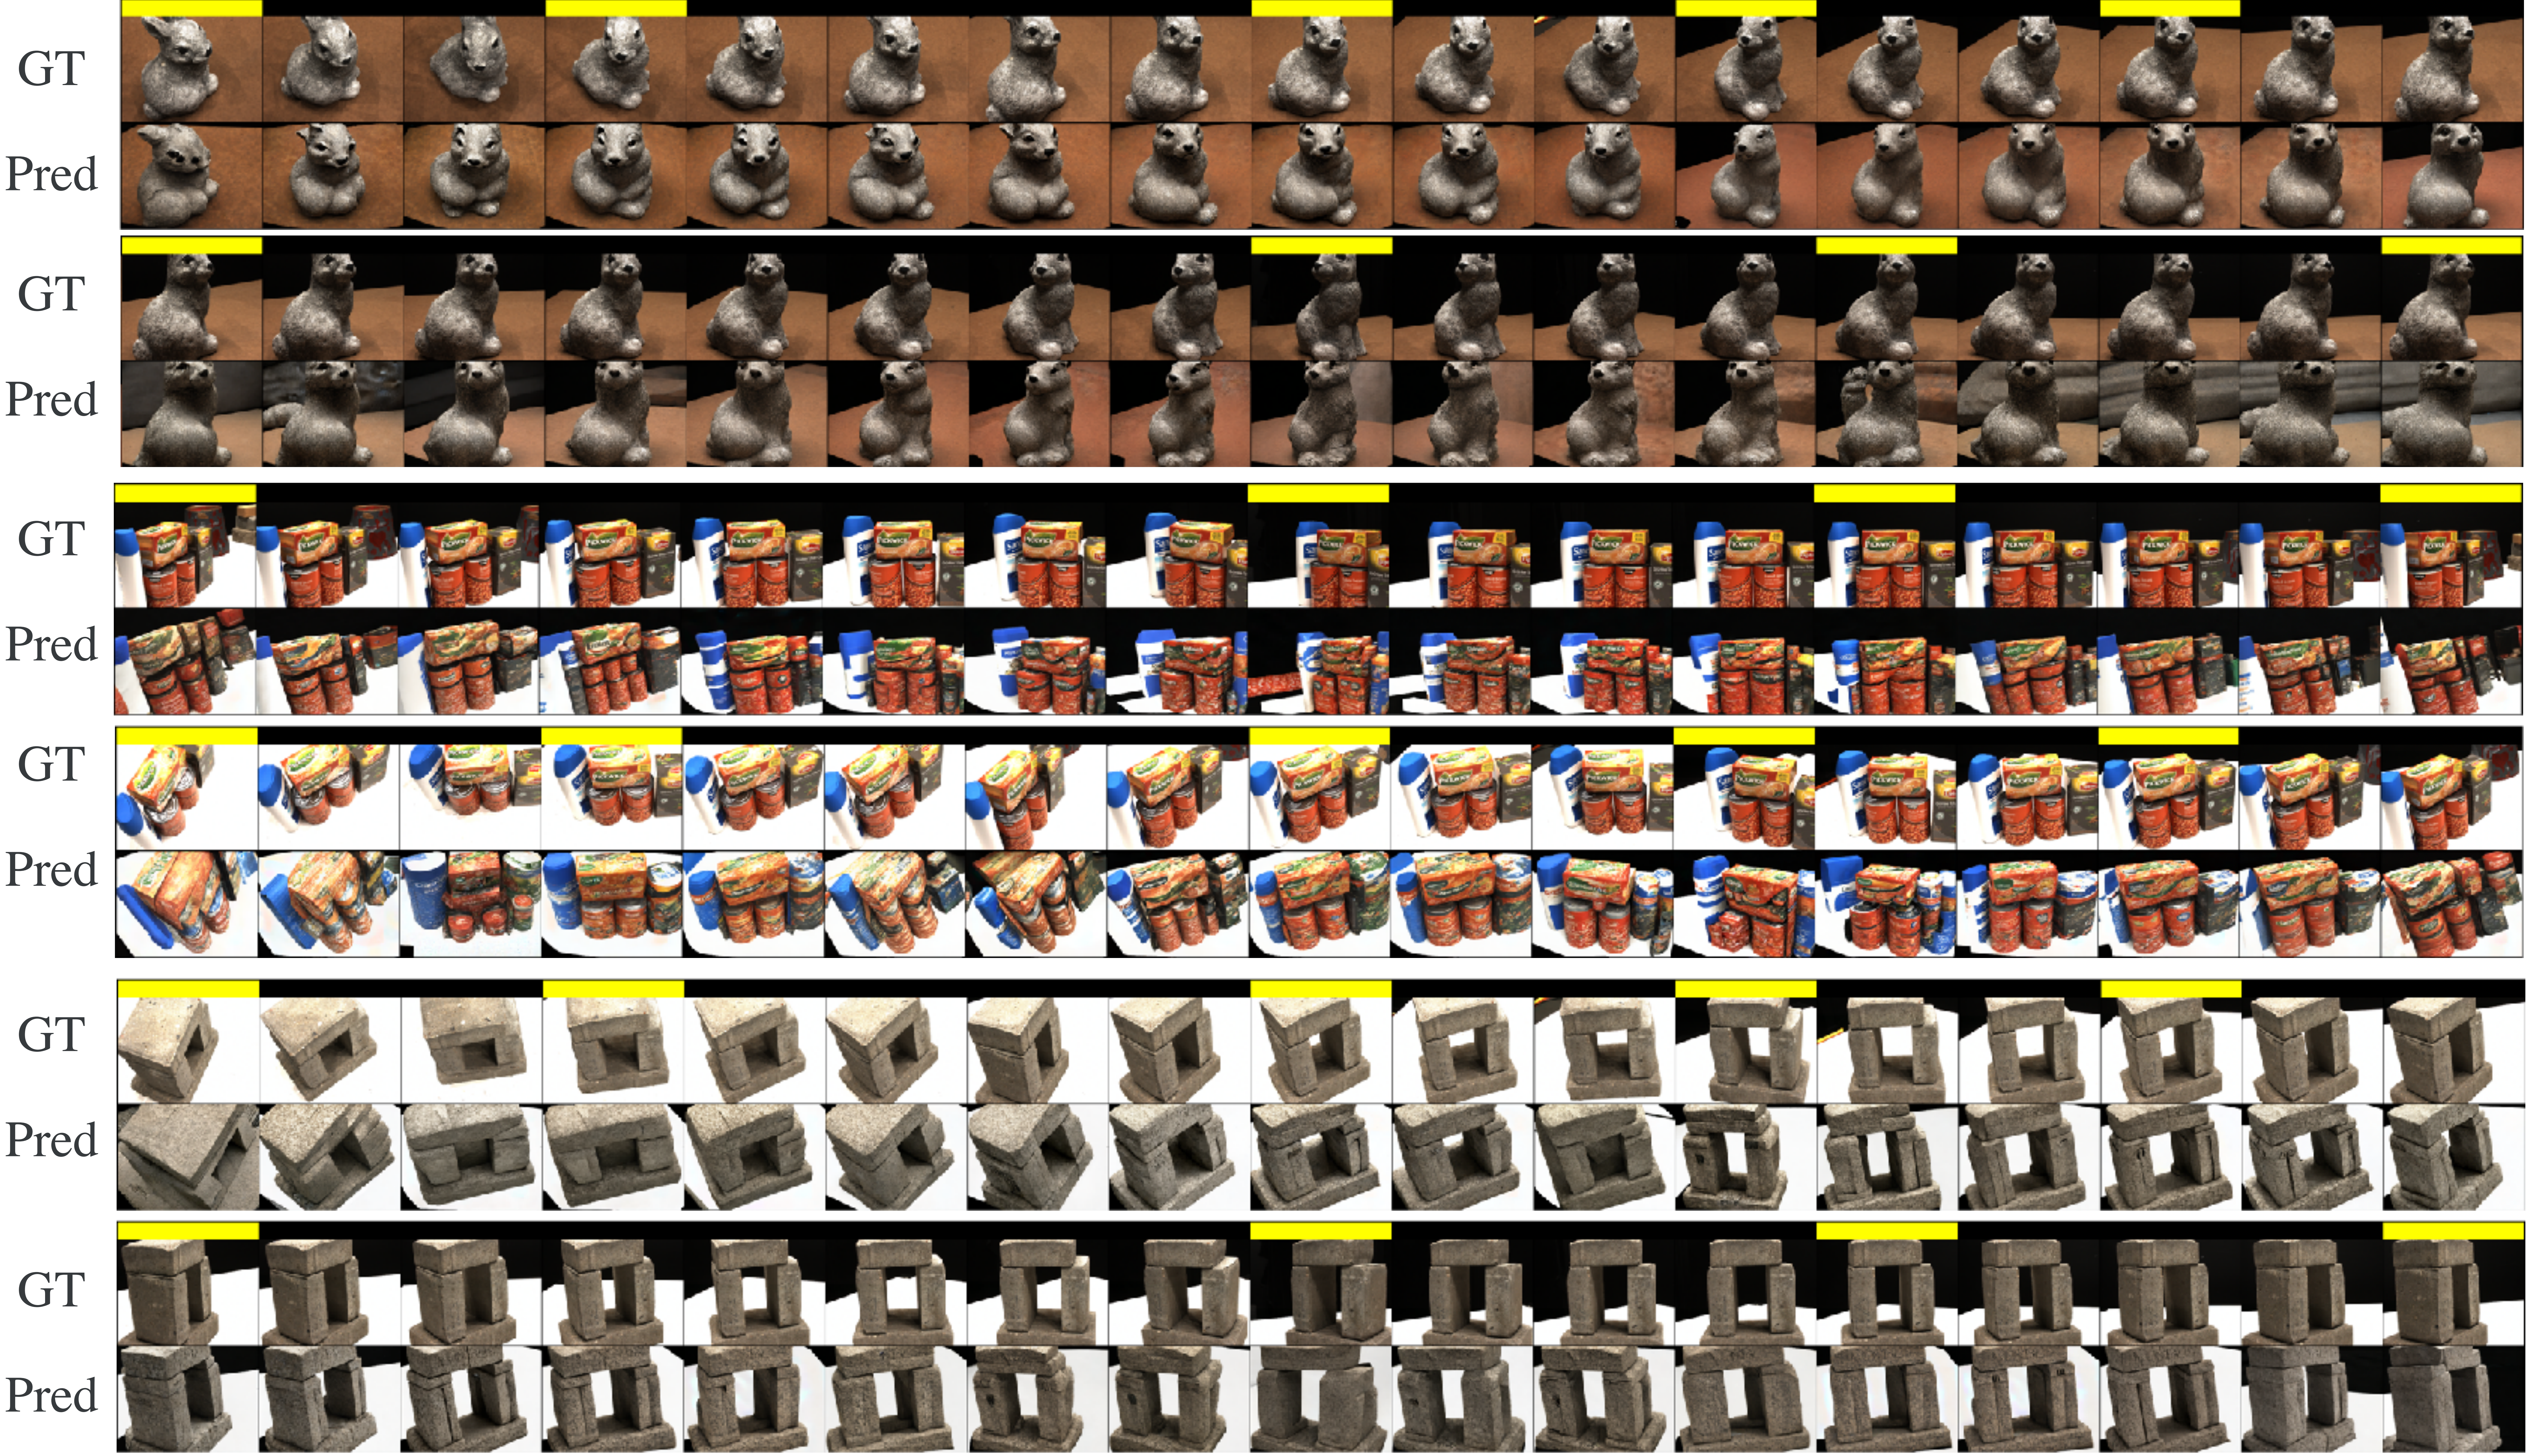


215

100

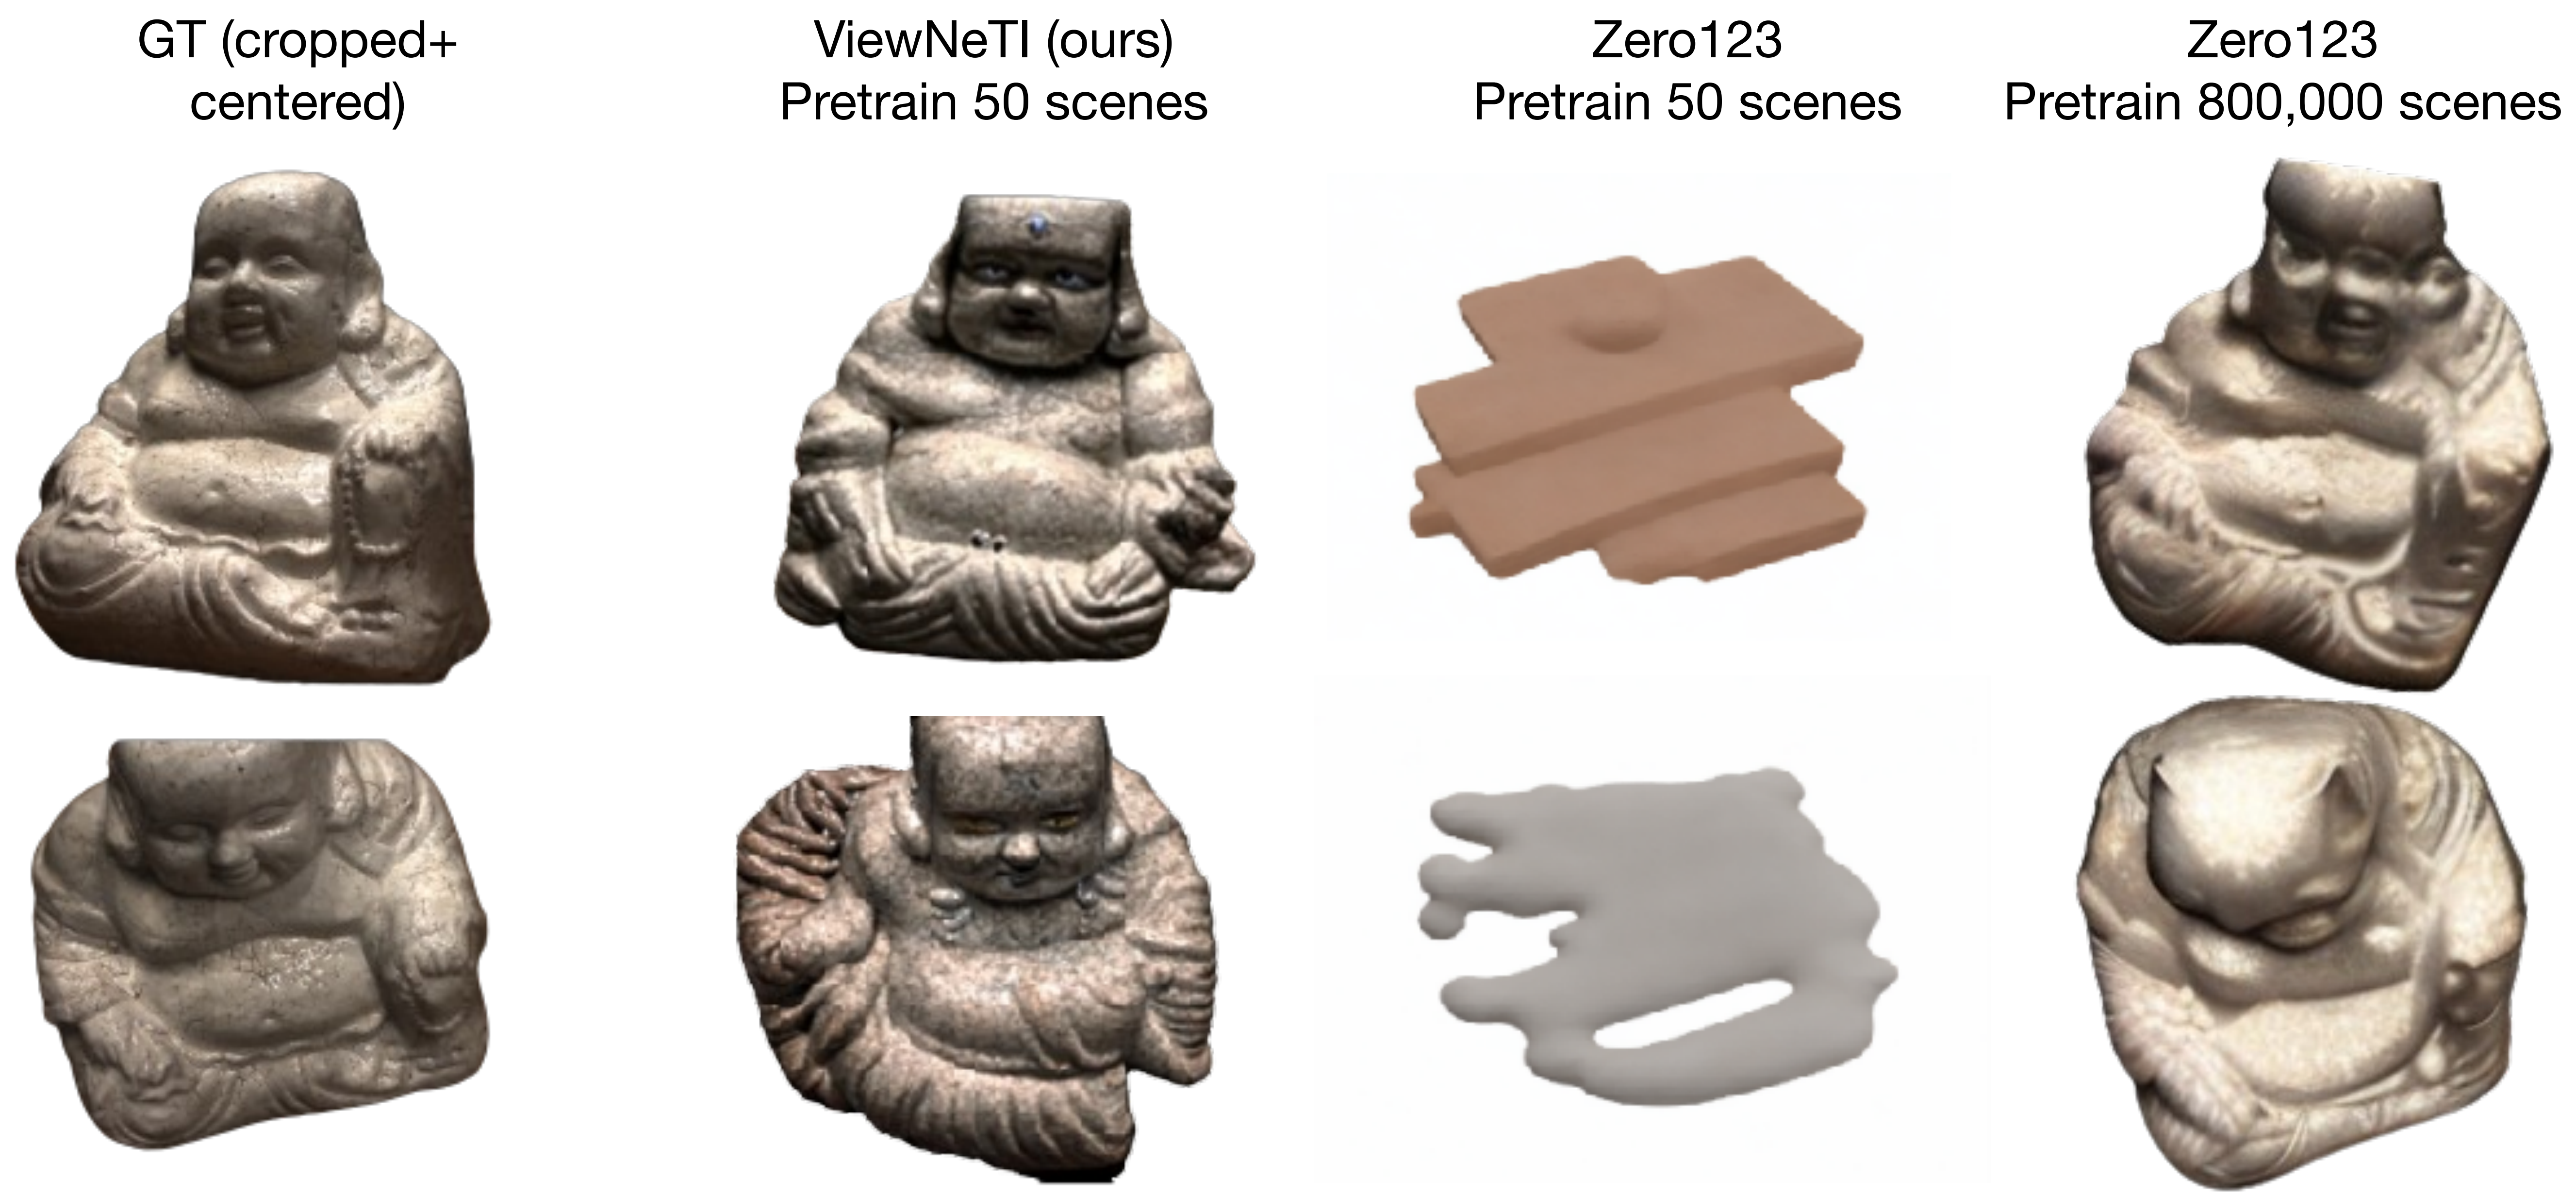
GT (cropped+ centered)
ViewNeTI (ours) Pretrain 50 scenes
Zero123 Pretrain 50 scenes
Zero123 Pretrain 800,000 scenes

850

605
